# Supplementary material for: Theory of Transport in Highly Concentrated Electrolytes
Source: arXiv:2010.14915 ancillary file (2022-01-10)
Supplement: Supplementary file 1 [file supplementary.pdf]

# Supplementary Information

# Theory of Transport in Highly Concentrated Electrolytes

Max Schammer,[1,2] Birger Horstmann,[1,2,3,*] and Arnulf Latz[1,2,3,†]

[1] *German Aerospace Center, Pfaffenwaldring 38-40, 70569 Stuttgart, Germany*

[2] *Helmholtz Institute Ulm, Helmholtzstraße 11, 89081 Ulm, Germany*

[3] *Universität Ulm, Albert-Einstein-Allee 47, 89081 Ulm, Germany*

## CONTENTS

SI 1. Theory 2

A. Symmetry Principles 2

B. Unification of Electromagnetic Theory with Mechanics and Thermodynamics 3

C. Symmetrization of the Viscosity Tensor 5

D. Constitutive Equation for the Chemical Potentials 7

E. Derivation of the Partial Molar Volumes from the Stress Tensor 8

F. Modelling Energy of Deformation 8

G. Transport Parameters in Different Reference Frames 8

H. Comment on Transference Numbers in Binary Electrolytes 12

I. Thermal Aspects 13

1. Heat Equation 13

2. Hydrodynamical Expansion 15

3. Thermal Model for the Free Energy Density 19

J. Matrix Formulation of the Transport Theory 21

1. Example: Quaternary, Electroneutral Electrolyte in Isothermal Case 24

K. Transformation of Reference Species 25

1. Transformation of Reduced Quantities 26

2. Transformation of Mass Fluxes 27

3. Transformation of Onsager Matrix and Transport Parameters 28

* birger.horstmann@dlr.de

† arnulf.latz@dlr.de

4. Example: Quaternary Electrolyte 29
L. Formalizing Chemical Reactions 31

SI 2. Modelling of Zinc Ion Battery 32
A. Electrolyte Composition 32
1. Reactions 32
2. Initial Concentrations 33
3. Partial Molar Volumes 34
4. Viscosity 34
5. Transport Parameters: Modelling Onsager Matrix 35
B. Electrodes 36
1. Solid Phase Equations 36
2. Electrode Parameters 37
C. Implementation: Computational Details 38

SI 3. Simulation Results 38
A. Electrolyte Dynamics 38
1. High Discharge Current 41
2. Various Currents 41
B. Consistency Check: Varying Reference Species 43

References 44

# SI 1. THEORY

## A. Symmetry Principles

In this work we assume the principle of "material frame-indifference", which is the classical equivalent to the principle of relativity. According to this universal constitutive principle, material functions associated to constitutive quantities must be form-invariant ("covariant") under Euclidean transformations.[1] Euclidean transformations comprise time-dependent orthogonal rotations and time-dependent translations, and represent arbitrary observer transformations.[2] In the limit of constant rotation and translation, they reduce to Galilei-transformations.[3] Also, the relativistic formulation of electromagnetism implies covariance with respect to Lorentz

transformations.[4] However, here we may safely assume the classical limit in which the convection velocity is negligible compared with the speed of light.[5] In this limit, Lorentz transformation reduces to Galilean transformation.[6]

Tensorial quantities which transform properly under Euclidean transformations are called *objective tensors*. For detailed definitions we refer to the literature, see ref. 7. Objectivity of kinematic quantities can be assessed analytically using the *representation theorems of isotropic tensors*.[8–10] For example, the velocity-gradient grad $\mathbf{v}$ is not objective, whereas the symmetrized strain-rate-tensor $\boldsymbol{\kappa}$ is objective.[1] Unlike the convection velocity $\mathbf{v}$, differences in velocities, like diffusion velocities $\mathbf{N}_\alpha$, are objective.[11] The electromagnetic quantities $\mathcal{J}, \mathcal{E}, \mathcal{H}, \mathbf{B}, \varrho, \mathbf{P}$ and $\mathbf{D}$ are also objective.[12] Again, we refer to the literature, for analytic proofs. In contrast, objectivity of non-kinematic tensorial quantities cannot always be assessed analytically. Thus, the transformation behaviour of such quantities (which include temperature, mass density, stress tensor, and the heat flux) must be postulated in analogy to experiments.[11]

Since the symmetry of linear constitutive equations depends on the transformation behaviour of the variables, we restrict the variable-set of our model $\boldsymbol{\Upsilon}$ ("*materials law*") to objective tensors.[12] However, any admissible set $\boldsymbol{\Upsilon}$ which consists of objective quantities is still subject to physical arguments, associated to the particular system of consideration. Thus, we do not use the complete set of objective variables in our electrolyte model.

Besides its abstract role in the materials law, we make explicit use of the symmetry-argument to find the correct expression for the viscosity tensor. The representation theorems for isotropic tensors uniquely determine the most general linear form of the (objective) viscosity-tensor $\boldsymbol{\tau}(\boldsymbol{\kappa})$, up to two scalar coefficients, see eq. (48).

Furthermore, we assume that the stress tensor is a symmetric matrix, $\boldsymbol{\sigma} = \boldsymbol{\sigma}^T$ (this assumption is not directly coupled to the principle of material frame indifference[6]). This excludes fluids with internal, rotational degrees of freedom (*e.g.*, spin) from our description.[11] Indeed, some ionic liquids exhibit spin-characteristics of liquid crystals, both in the bulk and/or in confined geometries.[13] However, here we do not resolve such microscopic details.

### B. Unification of Electromagnetic Theory with Mechanics and Thermodynamics

We assume that the time-evolution of the energy $\int \mathrm{d}V\, \rho\dot{\varepsilon} = \Pi + Q$ is determined by the powers of the forces acting on the system $\Pi$, and the heating of the system $Q$. The mechanical term is

related to the momentum-equation, $\Pi = \oint \mathrm{d}A\ \mathbf{v}(\boldsymbol{\sigma}\cdot\hat{\mathbf{n}}) + \int \mathrm{d}V\, \rho\mathbf{v}\mathbf{b}$. The heating $Q$ consists of a source-term $\rho h$ and a surface-flux of heat. We assume that, beneath the heat-conduction $-\mathbf{q}$, there exists an electromagnetic contribution $-(\mathcal{E}\wedge\mathcal{H})$, which acts on the system even when thermally insulated. Since all quantities appearing are assumed smooth, this leads to the local law of energy-balance eq. (9).

The quantity $\mathcal{E}\wedge\mathcal{H}$ is the Galilei-covariant expression of Poynting's vector. Here, we use Maxwell's equations in the covariant formulation

$$\nabla\mathbf{B} = 0, \qquad \overset{*}{\mathbf{B}} + \nabla\wedge\mathcal{E} = 0, \tag{SI 1}$$

$$\nabla\mathbf{D} = \varrho, \qquad \overset{*}{\mathbf{D}} - \nabla\wedge\mathcal{H} = -\mathcal{J}. \tag{SI 2}$$

The quantities $\varrho, \mathcal{J}$ are the free charge-/ flux-contributions, to which the dielectric displacement (potential) $\mathbf{D}$ is associated via eq. (SI 2)$_1$. The so-called flux-derivative of a vector field $\mathbf{m}$ appearing above is defined by $\overset{*}{\mathbf{m}} = \dot{\mathbf{m}} + \mathbf{m}(\nabla\mathbf{v}) - (\mathbf{m}\cdot\nabla)\,\mathbf{v}$, and describes the local time-evolution of a surface-field-density under time-dependent surface-boundaries.[6] From the Galilei-covariant description eq. (SI 1) follows that $\mathcal{H}(\nabla\wedge\mathcal{E}) = -\mathcal{H}\overset{*}{\mathbf{B}}$ and from the inhomogeneous eq. (SI 2) follows $\mathcal{E}(\nabla\wedge\mathcal{H}) = \mathcal{E}\dot{\mathbf{D}} + \mathcal{E}\mathcal{J}$. The identity $\nabla(\mathcal{H}\wedge\mathcal{E}) = \mathcal{E}(\nabla\wedge\mathcal{H}) - \mathcal{H}(\nabla\wedge\mathcal{E})$ then implies that the electromagnetic energy-flux satisfies $-\nabla(\mathcal{E}\wedge\mathcal{H}) = \mathcal{H}\overset{*}{\mathbf{B}} + \mathcal{E}\overset{*}{\mathbf{D}} + \mathcal{E}\mathcal{J}$. From the definition of the flux-derivative follows that for any two vector-fields $\mathbf{m}, \mathbf{n}$, the product $\mathbf{m}\overset{*}{\mathbf{n}} = \mathbf{m}\dot{\mathbf{n}} + [(\mathbf{m}\mathbf{n})\,\mathbf{Id} - \mathbf{m}\otimes\mathbf{n}] : \operatorname{grad}\mathbf{v}$. Hence, this yields the covariant identity

$$\nabla(\mathcal{H}\wedge\mathcal{E}) = \mathcal{H}\dot{\mathbf{B}} + \mathcal{E}\dot{\mathbf{D}} + \mathcal{E}\mathcal{J} + [(\mathcal{H}\mathbf{B} + \mathcal{E}\mathbf{D})\,\mathbf{Id} - \mathcal{H}\otimes\mathbf{B} - \mathcal{E}\otimes\mathbf{D}] : \operatorname{grad}\mathbf{v}. \tag{SI 3}$$

All tensor-terms appearing on the right side of eq. (SI 3) which are contracted with grad $\mathbf{v}$ contribute to the constitutive equation of the stress tensor, see eq. (24) and eq. (50). Thus, the stress tensor depends on the precise form of the electromagnetic contribution to the heating-flux. Furthermore, the expressions $\mathcal{E}\dot{\mathbf{D}}$ and $\mathcal{H}\dot{\mathbf{B}}$ appearing in eq. (SI 3) determine, together with the model for $\varphi_{\mathrm{H}}$, the electromagnetic constitutive equations, see eqs. (14) and (15), as well as eq. (19).

For example, an alternative choice is to use the polarization $\mathbf{P}$ instead of $\mathbf{D}$ (where $\mathbf{D} = \varepsilon_0\mathbf{E} + \mathbf{P}$) as electrostatic variable for $\varphi_{\mathrm{H}}$.[14] However, this implies that the expression for $\varphi_{\mathrm{H}}$ in eq. (14) must be altered to obtain the corresponding constitutive equation $\mathbf{P} = -\rho\,\partial\varphi_{\mathrm{H}}/\partial\mathcal{E}$,[6]

$$\varphi_{\mathrm{H}} = \varepsilon - Ts - \mathbf{g}\dot{\mathbf{v}} + \mathbf{v}^2\big/2 - \Big[\varepsilon_0\mathbf{E}^2\big/2 + \mathbf{B}^2\big/2\mu_0 + \mathcal{E}\mathbf{P} - \varepsilon_0\mathbf{E}\wedge\mathbf{B}\Big]\Big/\rho\,. \tag{SI 4}$$

This approach suggests the linear model $\mathbf{P} = \chi\varepsilon_0\mathbf{E}$, yielding $-\chi\varepsilon_0\mathbf{E}^2/2$ as electrostatic contribution

to $\rho\varphi_H$, which leads to an alternative constitutive equation for the stress tensor,

$$\boldsymbol{\sigma} = \frac{\mathcal{K}}{2}\left[1 - \left(\sum_{\alpha=1}^{N} c_\alpha \nu_\alpha\right)^2\right] \cdot \mathbf{Id} - \frac{\varepsilon_0 \chi}{2}\mathbf{E}^2 \cdot \mathbf{Id} + \mathbf{E} \otimes \mathbf{D} + \lambda \nabla \mathbf{v} \cdot \mathbf{Id} + 2\eta \boldsymbol{\kappa}_{\mathrm{tf}}. \tag{SI 5}$$

The evaluation of this model yields exactly the same constitutive transport equation eq. (65), as predicted by our model. Thus, both methodologies are equivalent. However, our approach with **D** as primary variable agrees with the standard definition for the electromagnetic energy, and the Maxwell stress tensor, see eqs. (17) and (54).

### C. Symmetrization of the Viscosity Tensor

The "mechanical" dissipation-term appearing in the entropy inequality eq. (15), $\boldsymbol{\tau} : \mathrm{grad}\,\mathbf{v}$, describes internal friction. In this work we neglect internal, rotational degrees of freedom (see also section SI 1 A), such that the viscosity tensor $\boldsymbol{\tau} = \boldsymbol{\sigma} - (\boldsymbol{\mathcal{E}} \otimes \mathbf{D} + \boldsymbol{\mathcal{H}} \otimes \mathbf{B}) + (\boldsymbol{\mathcal{E}}\mathbf{D} + \boldsymbol{\mathcal{H}}\mathbf{B} + \sum_{\alpha=1}^{N} \mu_\alpha c_\alpha - \rho\varphi_H)\,\mathbf{Id}$ is symmetric. This is exactly the case if the tensor-products $\boldsymbol{\mathcal{E}} \otimes \mathbf{D}$ and $\boldsymbol{\mathcal{H}} \otimes \mathbf{B}$ are symmetric. Although, this need not be the case in general, we will show that the coupling between $\boldsymbol{\mathcal{E}}$ and **D**, as well as between $\boldsymbol{\mathcal{H}}$ and **B**, implies exactly this property.

Apparently, the tensor-prodcuts $\boldsymbol{\mathcal{E}} \otimes \mathbf{D}$ and $\boldsymbol{\mathcal{H}} \otimes \mathbf{B}$ involve conjugate pairs of electromagnetic variables ($\boldsymbol{\mathcal{E}} = \partial(\rho\varphi_H)/\partial\mathbf{D}$ and $\boldsymbol{\mathcal{H}} = \partial(\rho\varphi_H)/\partial\mathbf{B}$). Thus, and because of the symmetry assumptions made in section SI 1 A, we can apply the following Lemma.

**Lemma 1** *Let $\Psi$ be a smooth function of a non-scalar variable* **Z**. *Then, $\Psi$ is invariant under orthogonal transformations $\boldsymbol{\mathcal{U}}$, $\Psi(\boldsymbol{\mathcal{U}}\mathbf{Z}) = \Psi(\mathbf{Z})$, if, and only if, the quantity $\mathbf{Z} \otimes \partial\Psi/\partial\mathbf{Z}$ is symmetric, i.e. if and only if the sum $\epsilon^{ijk} Z_i\, \partial\Psi \big/ \partial Z_j = 0$, for all spatial components $i, j, k$.*

**Proof:** Consider an infinitesimal orthogonal transformation, (*i.e.* a rotation), induced by a matrix $\boldsymbol{\mathcal{U}} \in SO(3)$, where $\boldsymbol{\mathcal{U}}^T = \boldsymbol{\mathcal{U}}^{-1}$ (orthogonality condition). From representation theory, we know that the generators of $SO(3)$ are anti-symmetric matrices. This can easily be verified by expanding the orthogonality condition up to second order in the infinitesimal representation $\boldsymbol{\mathcal{U}} = \mathbf{Id} + \varepsilon \cdot \boldsymbol{\omega}$,

$$\mathbf{Id} = \boldsymbol{\mathcal{U}}^T \cdot \boldsymbol{\mathcal{U}} = \left(\mathbf{Id} + \varepsilon \cdot \boldsymbol{\omega}^T\right) \cdot (\mathbf{Id} + \varepsilon \cdot \boldsymbol{\omega}) = \mathbf{Id} + \varepsilon\left(\boldsymbol{\omega} + \boldsymbol{\omega}^T\right) + O(\varepsilon^2).$$

Thus, in this approximation, the generators $\boldsymbol{\omega}$ are anti-symmetric matrices. Furthermore, since any anti-symmetric matrix has N(N-1)/2 independent components, and, here, N = 3, the genera-

tors $\boldsymbol{\omega}$ have three independent components. Thus, they are determined by the vector of angular-momentum $\boldsymbol{\Omega}$, via $\omega_{ij} = -\epsilon_{ijk}\boldsymbol{\Omega}comp^k$ (here $\epsilon_{ijk}$ is the Levi-Civita symbol).

To probe invariance of the field $\Psi(\mathbf{Z})$, we calculate the transformation behaviour of the argument, $\boldsymbol{\mathcal{U}}\mathbf{Z} = (\mathbf{Id} + \varepsilon\boldsymbol{\omega})\mathbf{Z} = \mathbf{Z} + \varepsilon\boldsymbol{\omega}\mathbf{Z}$. Since $\varepsilon\boldsymbol{\omega}\mathbf{Z} = -\varepsilon\mathbf{Z} \wedge \boldsymbol{\Omega}$, this becomes $\boldsymbol{\mathcal{U}}\mathbf{Z} = \mathbf{Z} - \varepsilon \cdot \mathbf{Z} \wedge \boldsymbol{\Omega}$. Therefore, $\Psi$ is invariant under orthogonal transformations if $\Psi(\mathbf{Z} - \epsilon \cdot \mathbf{Z} \wedge \boldsymbol{\Omega}) = \Psi(\mathbf{Z})$, or, equivalently, if $\partial\Psi(\boldsymbol{\mathcal{U}}\mathbf{Z})/\partial\boldsymbol{\Omega} = 0$. In particular, for any spatial component $i$,

$$
\begin{aligned}
\frac{\partial\Psi(\boldsymbol{\mathcal{U}}\mathbf{Z})}{\partial\Omega^i} &= \frac{\partial\Psi(\mathbf{Z} - \varepsilon \cdot \mathbf{Z} \wedge \boldsymbol{\Omega})}{\partial\Omega^i} \\
&= \frac{\partial\Psi}{\partial(\mathbf{Z} - \epsilon\mathbf{Z} \wedge \boldsymbol{\Omega})^j} \frac{\partial(\mathbf{Z} - \varepsilon\mathbf{Z} \wedge \boldsymbol{\Omega})^j}{\partial\Omega <^i} \\
&= -\frac{\partial\Psi}{\partial(\mathbf{Z} - \varepsilon\mathbf{Z} \wedge \boldsymbol{\Omega})^j} \cdot \varepsilon\epsilon_{jkl}\delta^l_i Z^k \\
&= \varepsilon\epsilon_{ikj} Z^k \frac{\partial\Psi}{\partial(\mathbf{Z} - \varepsilon\mathbf{Z} \wedge \boldsymbol{\Omega})^j}.
\end{aligned} \tag{SI 6}
$$

Without loss of generality, let us assume that $\boldsymbol{\Omega} = 0$. Then, the left hand side vanishes identically, $\partial\Psi/\partial\boldsymbol{\Omega}|_{\boldsymbol{\Omega}=0} = 0$, whereas the right hand side becomes a derivative with respect to $\mathbf{Z}$. Thus, $0 = \varepsilon\epsilon_{ikj}Z^k \cdot \partial\Psi/\partial Z^j$, which is true for arbitrary $i$, exactly if $Z^k \cdot \partial\Psi/\partial Z^j - Z^j \cdot \partial\Psi/\partial Z^k = 0$. This completes the proof.

■

Therefore, due to this Lemma, $\boldsymbol{\mathcal{E}} \otimes \mathbf{D} = \mathbf{D} \otimes \boldsymbol{\mathcal{E}}$ and $\boldsymbol{\mathcal{H}} \otimes \mathbf{B} = \mathbf{B} \otimes \boldsymbol{\mathcal{H}}$. Using the invariance of the contraction-operation under transposition, *i.e.* $\boldsymbol{\mathcal{M}} : \boldsymbol{\mathcal{N}} = \boldsymbol{\mathcal{M}}^T : \boldsymbol{\mathcal{N}}^T$ for any two matrices $\boldsymbol{\mathcal{M}}$ and $\boldsymbol{\mathcal{N}}$, we thus get

$$\boldsymbol{\mathcal{E}} \otimes \mathbf{D} : \mathrm{grad}\,\mathbf{v} = \frac{1}{2}\left(\boldsymbol{\mathcal{E}} \otimes \mathbf{D} : \mathrm{grad}\,\mathbf{v} + \mathbf{D} \otimes \boldsymbol{\mathcal{E}} : \mathrm{grad}\,\mathbf{v}\right) \tag{SI 7}$$

$$= \frac{1}{2}\left(\boldsymbol{\mathcal{E}} \otimes \mathbf{D} : \mathrm{grad}\,\mathbf{v} + \boldsymbol{\mathcal{E}} \otimes \mathbf{D} : \mathrm{grad}\,\mathbf{v}^T\right) \tag{SI 8}$$

$$= \boldsymbol{\mathcal{E}} \otimes \mathbf{D} : \boldsymbol{\kappa} \tag{SI 9}$$

$$= \frac{1}{2}\left(\boldsymbol{\mathcal{E}} \otimes \mathbf{D} + \mathbf{D} \otimes \boldsymbol{\mathcal{E}}\right) : \boldsymbol{\kappa}. \tag{SI 10}$$

Since the same argument holds for the product $\boldsymbol{\mathcal{H}} \otimes \mathbf{B}$, the mechanical dissipation appearing in eq. (15) becomes $\boldsymbol{\tau} : \mathrm{grad}\,\mathbf{v} = \boldsymbol{\tau} : \boldsymbol{\kappa}$.

### D. Constitutive Equation for the Chemical Potentials

In the main text, we derived the constitutive equations via a semi-phenomenologic approach. Alternatively, the set of constitutive equations eqs. (18) to (21) can be derived by application of the method of Coleman and Noll.[6] Since this method is commonly used throughout the literature, we briefly sketch that it yields the same results, when applied to our modelling framework.

The method of Coleman and Noll yields closure relations for the set of variables $s, \boldsymbol{\mathcal{E}}, \boldsymbol{\mathcal{H}}, \mu_\alpha, \kappa$ by the formal evaluation of $\dot{\varphi}_\mathrm{H}(\boldsymbol{\Upsilon}) = \sum_A \partial\varphi_\mathrm{H}/\partial\Upsilon_A \cdot \dot{\Upsilon}_A$ in the dissipation law eq. (15). Here, the materials law of the free energy density is $\boldsymbol{\Upsilon} = (T, \mathbf{D}, c_\alpha, \kappa)$. However, our materials law comprises redundant variables. Due to the electrolyte equation of state, only N-1 concentrations $c_\alpha$ in a N-component electrolyte are independent. Thus, the constitutive equations with respect to the redundant variables, *viz.* the chemical potentials, are not unique, when derived by the method of Coleman and Noll. However, it turns out that this ambiguity is none of a problem, since we formulate our transport equations the reduced chemical potentials $\tilde{\mu}_\alpha, \tilde{\tilde{\mu}}_\alpha$, which are unambiguous. In this section, we shall derive this property.

Usually, the materials law is reduced to the set of independent variables. In contrast, applying the method of Coleman and Noll to the redundnat set $\Upsilon$ yields a closure relation of the form, $\sum_{\alpha=1}^{\mathrm{N}}(\rho M_\alpha\, \partial\varphi_\mathrm{H}/\partial\rho_\alpha - \mu_\alpha)\boldsymbol{\nabla}\mathbf{N}_\alpha$, appearing in the dissipation law. This suggests constitutive equations $\mu_\alpha = \rho M_\alpha \partial\varphi_\mathrm{H}/\partial\rho_\alpha$, which are different from the canonic definition eq. (21). However, due to mass conservation, $\sum_{\alpha=1}^{\mathrm{N}} M_\alpha \mathbf{N}_\alpha = 0$, we can add any term $\sum_{\alpha=1}^{\mathrm{N}} \xi \cdot M_\alpha \boldsymbol{\nabla}\mathbf{N}_\alpha = 0$ to the closure relation above. Here, $\xi$ is some "gauge-factor" of dimension $\dim(\xi) = \dim(\varphi_\mathrm{H})$. Therefore, the corresponding constitutive equation has the free parameter $\xi$,

$$\mu_\alpha^\xi = M_\alpha \left( \xi + \rho \frac{\partial\varphi_\mathrm{H}}{\partial\rho_\alpha} \right). \tag{SI 11}$$

In particular, the choice $\xi = \varphi_\mathrm{H}$ leads to the canonical definition $\mu_\alpha^{\varphi_\mathrm{H}} = M_\alpha \partial(\rho\varphi_\mathrm{H})/\partial\rho_\alpha$. However, as we have shown, the chemical potentials appear in the transport equations in the form of $\tilde{\mu}_\alpha$ and $\tilde{\tilde{\mu}}_\alpha$, to which the ambiguity in the chemical potentials does not transfer; by definition, $\tilde{\mu}_\alpha = \mu_\alpha - \mu_1 M_\alpha/M_1$, such that

$$\tilde{\mu}_\alpha^\xi = M_\alpha \rho \frac{\partial\varphi_\mathrm{H}}{\partial\rho_\alpha} - M_1 \rho \frac{\partial\varphi_\mathrm{H}}{\partial\rho_1} = \mu_\alpha - \frac{M_\alpha}{M_1}\mu_1 = \tilde{\mu}_\alpha. \tag{SI 12}$$

As consequence, the quantities $\tilde{\mu}_\alpha$ (and thus the quantities $\tilde{\tilde{\mu}}_\alpha$) are independent of $\xi$. Hence, any choice $\xi$ will lead to the same results in the transport theory, and, thus, the ambiguity in the constitutive equations for the chemical potentials gets resolved.

Therefore, since we use the potentials $\tilde{\mu}_\alpha$ in the transport equations, our approach in the main part yields the same transport equations like the method of Coleman and Noll.

### E. Derivation of the Partial Molar Volumes from the Stress Tensor

By construction, pressure is a function of the materials law of the free energy density, $p = f(\mathcal{N}_\alpha/V, T, \mathbf{D})$. This implicitely defines volume as function $V(\mathcal{N}_\alpha, p, T, \mathbf{D})$. The derivative with respect to particle numbers, $\partial/\partial\mathcal{N}_\alpha|_{p,T,\mathbf{D}}$ (where $p$,$T$,$\mathbf{D}$ are kept constant),

$$0 = \frac{\partial p}{\partial \mathcal{N}_\alpha}|_{p,T,\mathbf{D}} \tag{SI 13}$$

$$= \sum_{\beta=1}^{\mathrm{N}} \frac{\partial f}{\partial c_\beta} \cdot \frac{\partial c_\beta}{\partial \mathcal{N}_\alpha} - \sum_{\beta=1}^{\mathrm{N}} \frac{\partial f}{\partial c_\beta} \cdot \frac{\partial c_\beta}{\partial V} \cdot \frac{\partial V}{\partial \mathcal{N}_\alpha} = \frac{\partial f}{\partial c_\alpha} \cdot \frac{1}{V} - \sum_{\beta=1}^{\mathrm{N}} \frac{\partial f}{\partial c_\beta} \cdot \frac{\mathcal{N}_\beta}{V^2} \cdot \frac{\partial V}{\partial \mathcal{N}_\alpha}. \tag{SI 14}$$

This allows to solve for the partial molar volume,

$$\nu_\alpha = \frac{\partial V}{\partial \mathcal{N}_\alpha} = \frac{\partial p/\partial c_\alpha}{\sum_{\beta=1}^{\mathrm{N}} c_\beta \cdot \partial p/\partial c_\beta}. \tag{SI 15}$$

### F. Modelling Energy of Deformation

Let $\Psi(V, p, T)$ be the contribution to the free energy density stemming from volume-deformations. We model this quantity assuming a linear response to volume-perturbations around a stable reference state $\Psi^R(V^R, p^R, T^R)$, where the energy of deformation is minimal. Without loss of generality, we set $\Psi^R = 0$. As $\partial\Psi/\partial V|_{V^R} = 0$ (stability criterion), the first nonvanishing contribution to the Taylor-expansion of $\Psi$ is the second order,

$$\Psi(V^R + \varepsilon) = \frac{1}{2}\frac{\partial^2 \Psi}{\partial V^2}|_{V^R} \cdot \left(V - V^R\right)^2, \tag{SI 16}$$

where $V = V^R + \varepsilon$, and $\varepsilon \ll V^R$. In the main text, we show that $\mathcal{K} = V^2 \cdot \partial^2\Psi/\partial V^2|_{V^R}$ is indeed the bulk modulus in the case of incompressible electrolytes, see eq. (59).

### G. Transport Parameters in Different Reference Frames

In the main text, we developed our transport theory relative to the center-of-mass frame (CMF), and employed fluxes $\mathbf{N}_\alpha = c_\alpha(\mathbf{v}_\alpha - \mathbf{v})$. This approach has the advantage that it implies the trivial flux constraint $\sum_\alpha M_\alpha \mathbf{N}_\alpha = 0$. We made use of this description, and reduced the number of independent quantities $\mathbf{N}_\alpha$ to N-1.

The choice of the fluxes determines the reference-system of the transport theory. In general, two types of frames exist. In dynamic frames, the reference depends on the dynamics of the electrolyte, as it is defined relative to some set of “internal coordinates”. Alternatively, in static frames, the reference is defined by fixed external coordinates of the laboratory-frame (LF), which are independent of the electrolyte-dynamics. The CMF is an internal frame where convection serves as reference-velocity.

In the following, we sketch three alternative reference-frames, and evaluate each frame using thermodynamically consistent Onsager Ansatzes. This implies varying formulations of the respective transport coefficients. However, all of them are related by simple transformation rules between the individual frames.

Principal quantity for the development of the transport theory in all frames is the flux-part of the entropy inequality eq. (24),

$$\mathcal{R}^{\text{flux}} = -\sum_{\alpha=1}^{N} \mathbf{N}_\alpha \cdot \boldsymbol{\nabla}\mu_\alpha - \boldsymbol{\mathcal{J}} \cdot \boldsymbol{\nabla}\Phi = -\sum_{\alpha=1}^{N} \mathbf{N}_\alpha \cdot \boldsymbol{\nabla}\mu_\alpha^{\text{el}}, \tag{SI 17}$$

which determines the corresponding thermodynamically consistent Onsager coefficients. In the main text we introduced a reduction-mechanism for valencies and chemical potentials, stemming from mass-penalties relative to the designated species. Somewhat similar reduction-mechanisms arise when different constraints are evaluated. In general, constraints reduce the expansion of the entropy production $\mathcal{R}^{\text{flux}}$. This implies reduced sets of N-1 transference numbers parameters in internal frames, whereas N transference numbers exist in external frames. However, transference numbers sum up to one, hence only N-2 (N-1) independent transference numbers exist in internal (external) frames.

Here, we want to demonstrate that one can transform between different reference systems. Therefore, we restrict our discussion to the case of vanishing viscous forces $\boldsymbol{\nabla\tau} = 0$. In this case, assuming mechanical equilibrium ($\boldsymbol{\nabla\sigma} = 0$) yields a trivial Gibbs-Duhem relation $\sum_{\alpha=1}^{N} c_\alpha \cdot \boldsymbol{\nabla}\mu_\alpha^{\text{el}} = \boldsymbol{\nabla\tau} = 0$. This implies that the flux-term becomes

$$\mathcal{R}^{\text{flux}} = -\sum_{\alpha=1}^{N} \mathbf{N}_\alpha \cdot \boldsymbol{\nabla}\mu_\alpha^{\text{el}} = -\sum_{\alpha=1}^{N} \mathbf{n}_\alpha \cdot \boldsymbol{\nabla}\mu_\alpha^{\text{el}}. \tag{SI 18}$$

***External frame (LF):*** The simplest frame is defined by the N fluxes $\mathbf{n}_\alpha = c_\alpha \mathbf{v}_\alpha$. For this most basic external frame, we do not apply any constraint on the fluxes $\mathbf{n}_\alpha$. Thus, the sum in eq. (SI 18) is not reduced. We ensure non-negativity of $\mathcal{R}^{\text{flux}}$ using the Onsager Ansatz $\mathbf{n}_\alpha = -\sum_{\beta=1}^{N} \mathcal{L}_{\alpha\beta}^{\text{LF}} \cdot \boldsymbol{\nabla}\mu_\beta^{\text{el}}$.

In this frame, the transport parameters are

$$\kappa^{\mathrm{LF}} = F^2 \sum_{\alpha,\beta=1}^{\mathrm{N}} \mathcal{L}^{\mathrm{LF}}_{\alpha\beta} z_\alpha z_\beta, \quad t^{\mathrm{LF}}_\alpha = \frac{F^2}{\kappa^{\mathrm{LF}}} \sum_{\beta=1}^{\mathrm{N}} \mathcal{L}^{\mathrm{LF}}_{\alpha\beta} z_\alpha z_\beta, \quad \mathcal{D}^{\mathrm{LF}}_{\alpha\beta} = \mathcal{L}^{\mathrm{LF}}_{\alpha\beta} - \kappa^{\mathrm{LF}} \frac{t^{\mathrm{LF}}_\alpha t^{\mathrm{LF}}_\beta}{F^2 z_\alpha z_\beta}, \tag{SI 19a}$$

and the fluxes become

$$\boldsymbol{j} = -\kappa^{\mathrm{LF}} \nabla\Phi - F \sum_{\alpha,\beta=1}^{\mathrm{N}} \mathcal{L}^{\mathrm{LF}}_{\alpha\beta} z_\alpha \nabla\mu_\beta, \quad \mathbf{n}_\alpha = \frac{t^{\mathrm{LF}}_\alpha}{F z_\alpha}\boldsymbol{j} - \sum_{\beta=1} \mathcal{D}^{\mathrm{LF}}_{\alpha\beta} \nabla\mu_\beta \tag{SI 19b}$$

Only N-1 transference numbers $t^{\mathrm{LF}}_\alpha$ are independent in this frame, as they obey the normalization condition $\sum_{\alpha=1}^{\mathrm{N}} t^{\mathrm{LF}}_\alpha = 1$.

***External volume reference frame (EVRF):*** A hybrid frame follows from the LF by applying the volume-constraint imposed by the elctrolyte-equation-of-state ($\sum_{\alpha=1}^{\mathrm{N}} \nu_\alpha c_\alpha = 1$). Conservation of volume-fractions in the fixed frame (which follows from the constitutive equation for convection, eq. (61)), $\sum_{\alpha=1}^{\mathrm{N}} \nu_\alpha \nabla\mathbf{n}_\alpha = 0$ reduces the number of independent fluxes. Assuming no-flux boundary conditions allows to designate one species-flux, $\mathbf{n}_\delta = -\sum_{\alpha\neq\delta}^{\mathrm{N}} \nu_\alpha/\nu_\delta \cdot \mathbf{n}_\alpha$, which serves as reference. Here, the reduction mechanism comes in the form of volume-ratios and is similar to the mass-ratios used in the CMF-reduction-mechanism. This suggests definitions $\bar{z}^{(\delta)}_\alpha = z_\alpha - \nu_\alpha/\nu_\delta \cdot z_\delta$, $\bar{\mu}^{(\delta)}_\alpha = \mu_\alpha - \nu_\alpha/\nu_\delta \cdot \mu_\delta$, such that $\mathcal{R} = -\sum_{\alpha\neq\delta}^{\mathrm{N}} \mathbf{n}_\alpha \cdot \nabla\bar{\mu}^{(\delta);\mathrm{el}}_\alpha$, where $\bar{\mu}^{(\delta);\mathrm{el}}_\alpha = F\bar{z}^{(\delta)}_\alpha \nabla\Phi + \nabla\bar{\mu}^{(\delta)}_\alpha$. The Onsager-Ansatz $\mathbf{n}_\alpha|_{\alpha\neq\delta} = -\sum_{\beta\neq\delta}^{\mathrm{N}} \bar{\mathcal{L}}^{(\delta)}_{\alpha\beta} \bar{\mu}^{(\delta);\mathrm{el}}_\beta$ ensures non-negativity of $\mathcal{R}^{\mathrm{flux}}$. We expand the electric current in this frame, yielding transport parameters

$$\bar{\kappa}^{(\delta)} = F^2 \sum_{\alpha,\beta\neq\delta} \bar{\mathcal{L}}^{(\delta)}_{\alpha\beta} \bar{z}^{(\delta)}_\alpha \bar{z}^{(\delta)}_\beta, \quad \bar{t}^{(\delta)}_\alpha = \frac{F^2}{\bar{\kappa}} \sum_{\beta\neq\delta}^{\mathrm{N}} \bar{\mathcal{L}}^{(\delta)}_{\alpha\beta} \bar{z}^{(\delta)}_\alpha \bar{z}^{(\delta)}_\beta, \quad \bar{\mathcal{D}}^{(\delta)}_{\alpha\beta} = \bar{\mathcal{L}}^{(\delta)}_{\alpha\beta} - \bar{\kappa}^{(\delta)} \frac{\bar{t}^{(\delta)}_\alpha \bar{t}^{(\delta)}_\beta}{F^2 \bar{z}^{(\delta)}_\alpha \bar{z}^{(\delta)}_\beta}, \tag{SI 20a}$$

and fluxes

$$\boldsymbol{j} = -\bar{\kappa}^{(\delta)} \nabla\Phi - \sum_{\alpha\beta\neq\delta}^{\mathrm{N}} F \bar{\mathcal{L}}^{(\delta)}_{\alpha\beta} \bar{z}^{(\delta)}_\alpha \nabla\bar{\mu}^{(\delta)}_\alpha, \text{ and } \mathbf{n}_\alpha = \frac{\bar{t}^{(\delta)}_\alpha}{F\bar{z}^{(\delta)}_\alpha}\boldsymbol{j} - \sum_{\beta\neq\delta} \bar{\mathcal{D}}^{(\delta)}_{\alpha\beta} \nabla\bar{\mu}^{(\delta)}_\beta. \tag{SI 20b}$$

Note that only N-2 independent coefficients $\bar{t}^{(\delta)}_\alpha$ exist, as the N-1 parameters obey the normalization condition $\sum_{\alpha\neq\delta}^{\mathrm{N}} \bar{t}^{(\delta)}_\alpha = 1$. This frame is intermediate in the sense that it is based on the LF-fluxes although an internal, but not dynamical quantity ($\nu_\alpha/\nu_\delta$) is used as reduction-agent. Also, only N-1×N-2 coefficients $\bar{\mathcal{D}}^{(\delta)}_{\alpha\beta}$ are independent, as they obey trivial relations $\sum_{\beta\neq\delta} \bar{\mathcal{D}}^{(\delta)}_{\alpha\beta} \bar{z}^{(\delta)}_\beta$=0, hence $\bar{\mathcal{D}}^{(\delta)}_{\alpha\sigma}$=-$\sum_{\beta\neq\delta,\sigma} \bar{\mathcal{D}}^{(\delta\sigma)}_{\alpha\beta} \cdot \bar{z}^{(\delta)}_\beta / \bar{z}^{(\delta)}_\sigma$. Therefore,

$$\mathbf{n}_\alpha = \frac{\bar{t}^{(\delta)}_\alpha}{F\bar{z}^{(\delta)}_\alpha}\boldsymbol{j} - \sum_{\beta\neq\delta,\sigma} \bar{\mathcal{D}}^{(\delta\sigma)}_{\alpha\beta} \nabla\bar{\bar{\mu}}^{(\delta\sigma)}_\beta, \text{ where } \bar{\bar{\mu}}^{(\delta\sigma)}_\beta = \bar{\mu}^{(\delta)}_\beta - \frac{\bar{z}^{(\delta)}_\beta}{\bar{z}^{(\delta)}_\sigma} \bar{\mu}^{(\delta)}_\sigma. \tag{SI 21}$$

The transfer-relations between the two frames for the diffuion coefficients and the maximally reduced potentials $\bar{\bar{\mu}}_\alpha$ and $\tilde{\tilde{\mu}}_\alpha$ follow by assuming vanishing current $\mathcal{J}$=0,

$$\sum_{\beta\neq\delta,\sigma} \bar{\mathcal{D}}^{(\delta\sigma)}_{\alpha\beta} \boldsymbol{\nabla} \bar{\bar{\mu}}^{(\delta\sigma)}_\beta = \sum_{\beta=3} \mathcal{D}^{\text{CMF}}_{\alpha\beta} \boldsymbol{\nabla} \tilde{\tilde{\mu}}_\beta - c_\alpha \mathbf{v}, \tag{SI 22}$$

$$\bar{\bar{\mu}}^{(\delta\sigma)}_\beta = \tilde{\tilde{\mu}}_\beta + \left( \frac{M_\beta + M_2 \tilde{z}_\beta / \tilde{z}_2}{M_1} - \frac{\nu_\beta + \nu_\sigma \tilde{z}_\beta / \tilde{z}_2}{\nu_\delta} \right) \mu_1. \tag{SI 23}$$

In this frame, we used a volumetric constraint to reduce the number of independent species by one. However, it is not so clear how to reduce the number of independent species further. Thus, in principle, it is not clear how to ensure momentum-conservation in this frame. Therefore, the CMF-formulation of the transport theory has conceptual advantages. Momentum conservation is directly cast into the framework and allows to derive an equation for **v**. Furthermore, the coupling to mechanics and viscosity emerges naturally in the CMF. The external frame is advantageous when the center-of-mass motion vanishes.

***Internal velocity reference frame (IVRF):*** We construct an internal frame similar to the CMF using the specific velocity of one designated species, instead of the convection, for the reference-velocity. Thus, we define N-1 $\breve{\mathbf{N}}^{(\gamma)}_\alpha = c_\alpha \left( \mathbf{v}_\alpha - \mathbf{v}_\gamma \right) = \mathbf{n}_\alpha - c_\alpha \mathbf{v}_\gamma$. In this frame, the entropy production rate becomes,

$$\mathcal{R} = -\sum_{\alpha=1}^{\text{N}} \mathbf{n}_\alpha \boldsymbol{\nabla} \mu^{\text{el}}_\alpha = -\sum_{\alpha\neq\gamma}^{\text{N}} \breve{\mathbf{N}}^{(\gamma)}_\alpha \boldsymbol{\nabla} \mu^{\text{el}}_\alpha + \mathbf{v}_\gamma \sum_{\alpha=1}^{\text{N}} c_\alpha \boldsymbol{\nabla} \mu^{\text{el}}_\alpha = -\sum_{\alpha\neq\gamma}^{\text{N}} \breve{\mathbf{N}}^{(\gamma)}_\alpha \boldsymbol{\nabla} \mu^{\text{el}}_\alpha, \tag{SI 24}$$

where we used the trivial Gibbs-Duhem relation. This becomes non-negative by the Onsager Ansatz $\breve{\mathbf{N}}^{(\gamma)}_\alpha = -\sum^{\text{N}}_{\beta\neq\gamma} \breve{\mathcal{L}}^{(\gamma)}_{\alpha\beta} \boldsymbol{\nabla} \mu^{\text{el}}_\beta$. In this frame, the transport parameters become

$$\breve{\kappa}^{(\gamma)} = F^2 \sum_{\alpha,\beta\neq\gamma}^{\text{N}} \breve{\mathcal{L}}^{(\gamma)}_{\alpha\beta} z_\alpha z_\beta, \quad \breve{t}^{(\gamma)}_\alpha = \frac{F^2}{\breve{\kappa}^{(\gamma)}} \sum_{\beta\neq\gamma} \breve{\mathcal{L}}^{(\gamma)}_{\alpha\beta} z_\alpha z_\beta, \quad \breve{\mathcal{D}}^{(\gamma)}_{\alpha\beta} = \breve{\mathcal{L}}^{(\gamma)}_{\alpha\beta} - \breve{\kappa}^{(\gamma)} \frac{\breve{t}^{(\gamma)}_\alpha \breve{t}^{(\gamma)}_\beta}{F^2 z_\alpha z_\beta}, \tag{SI 25a}$$

whereas the fluxes become

$$\boldsymbol{j} = -\breve{\kappa}^{(\gamma)} \boldsymbol{\nabla} \Phi - \sum_{\alpha,\beta\neq\gamma}^{\text{N}} \breve{\mathcal{L}}^{(\gamma)}_{\alpha\beta} z_\alpha \boldsymbol{\nabla} \mu_\beta + \varrho \mathbf{v}_\gamma, \;\text{ and }\; \breve{\mathbf{N}}^{(\gamma)}_\alpha = \frac{\breve{t}^{(\gamma)}_\alpha}{F z_\alpha} \left( \boldsymbol{j} - \varrho \mathbf{v}_\gamma \right) - \sum_{\beta\neq\gamma}^{\text{N}} \breve{\mathcal{D}}^{(\gamma)}_{\alpha\beta} \mu_\beta. \tag{SI 25b}$$

As in all internal frames, only N-2 transference numbers $\breve{t}^{(\gamma)}_\alpha$ are independent, since they obey the normalization $\sum^{\text{N}}_{\alpha\neq\gamma} \breve{t}^{(\gamma)}_\alpha = 1$.

***Transformation rules:*** Assuming chemical equilibrium allows to compare the conductivities of the respective frames,

$$\kappa^{\text{LF}} = \bar{\kappa}^{(\delta)} = \breve{\kappa}^{(\gamma)} + \varrho \cdot \frac{\mathbf{v}_\gamma \mathbf{E}}{\mathbf{E}^2} = \kappa^{\text{CMF}} + \varrho \cdot \frac{\mathbf{v}\mathbf{E}}{\mathbf{E}^2}. \tag{SI 26}$$

Thus, the conductivities of both external frames are equal. Furthermore, in the electroneutral case ($\varrho = 0$) all electrolyte electric conductivities are equal. As expected, $\kappa^{\text{CMF}} = \kappa^{\text{LF}}$ if convection is negligible. Interestingly, if the reference motion is normal to the electric field (to the Lorentz-force), $(\mathbf{v}_\gamma, \mathbf{v}) \perp \mathbf{E}$, then all electrolyte conductivities are equal.

The complete set of transference numbers in one frame can be calculated from the complete set of parameters in any other frame. We summarize the transformation rules (here $t_\alpha$ are the transference numbers relative to the CMF, see eq. (39)),

$$t_\alpha^{\text{LF}}|_{\alpha\neq 1} = \frac{z_\alpha}{\tilde{z}_\alpha} t_\alpha \left(1 - \varrho \cdot \frac{\mathbf{v}\hat{\mathbf{e}}_j}{\sqrt{\boldsymbol{j}^2}}\right) + F c_\alpha z_\alpha \cdot \frac{\mathbf{v}\hat{\mathbf{e}}_j}{\sqrt{\boldsymbol{j}^2}}, \quad t_1^{\text{LF}} = 1 - \sum_{\alpha=2}^{\text{N}} t_\alpha^{\text{LF}}, \tag{SI 27}$$

$$\breve{t}_\alpha^{(\gamma)}|_{\alpha\neq\gamma} = t_\alpha^{\text{LF}} - \frac{z_\alpha c_\alpha}{z_\gamma c_\gamma} t_\gamma^{\text{LF}}, \tag{SI 28}$$

$$\bar{t}_\alpha^{(\delta)}|_{\alpha\neq\delta} = \frac{\bar{z}_\alpha^{(\delta)}}{z_\alpha} t_\alpha^{\text{LF}} = \left(1 - \frac{\nu_\alpha z_\delta}{\nu_\delta z_\alpha}\right) t_\alpha^{\text{LF}}. \tag{SI 29}$$

Note the deviation of the IVRF-transference numbers from the LF-parameters, eq. (SI 28). If the electrolyte consists of a binary salt with common anion (cation) $Y$, then the electroneutral correction for both cations (anions) is $\breve{t}_\alpha^{(Y)}|_{\alpha\neq Y} = t_\alpha^{\text{LF}} + c_\alpha/c^Y \cdot t_Y^{\text{LF}}$. For an abundant, charged designated species ($c_\delta \gg c_\alpha \forall\alpha \neq \delta$, $z_\delta \neq 0$), the correction is small. If the designated species is neutral, then the transference numbers in both external frames are equal, eq. (SI 29).

### H. Comment on Transference Numbers in Binary Electrolytes

In an electrolyte composed of N species, a total of N-1 transference numbers are defined in the CMF, whereas only N-2 are independent. However, a phenomenologic transference number of the designated species can be constructed using $\mathbf{N}_1 = -\sum_{\alpha=2}^{\text{N}} M_\alpha/M_1 \cdot \mathbf{N}_\alpha$. In chemical and thermal equilibrium, $\mathbf{N}_\alpha|_{\alpha\geq 2} = t_\alpha/F\tilde{z}_\alpha \cdot \mathcal{J}$, such that

$$\mathbf{N}_1 = -\sum_{\alpha=2}^{\text{N}} \frac{M_\alpha}{M_1} \frac{t_\alpha}{F\tilde{z}_\alpha} \cdot \mathcal{J}. \tag{SI 30}$$

By analogy, we construct the phenomenological parameter $\tau^{\text{CMF}}$ via $\mathbf{N}_1 = \tau^{\text{CMF}}/Fz_1 \cdot \mathcal{J}$. Thus, $\tau^{\text{CMF}}$ is a function of the transference numbers in the CMF, all masses and the valencies,

$$\tau^{\text{CMF}} = -\sum_{\alpha=2}^{\text{N}} \frac{M_\alpha}{M_1} \cdot \frac{z_1}{\tilde{z}_\alpha} \cdot t_\alpha = -\sum_{\alpha=2}^{\text{N}} \frac{M_\alpha z_1}{M_1 z_\alpha - M_\alpha z_1} \cdot t_\alpha = \sum_{\alpha=2}^{\text{N}} \left(1 - \frac{M_1 z_\alpha}{M_\alpha z_1}\right)^{-1} t_\alpha. \tag{SI 31}$$

For binary electrolytes, the ambiguity of internal transference becomes apparent, as, in this case, there is no independent transference number in the CMF at all. In particular, the only defined transference number is fixed, $t_2 = 1$. However, the phenomenological parameter above becomes

$$\tau^{\mathrm{CMF}} = \frac{M_2}{M_1 + M_2}, \tag{SI 32}$$

and is thus determined by the molar masses alone ("Sundheim's Golden rule").[15]

In contrast, exactly one independent external transference number exists in a binary electrolyte. It can be calculated from the CMF-parameter, $t_2 = 1$, and using eq. (SI 27). In particular,

$$t_2^{\mathrm{LF}} = \frac{M_2}{M_1 + M_2} - \frac{F z_1 \rho}{M_1 + M_2} \cdot \frac{\mathbf{v} \cdot \hat{\mathbf{e}}_j}{\sqrt{\boldsymbol{j}^2}} = \tau^{\mathrm{CMF}} - \frac{F z_1 \rho}{M_1 + M_2} \cdot \frac{\mathbf{v} \cdot \hat{\mathbf{e}}_j}{\sqrt{\boldsymbol{j}^2}}, \tag{SI 33}$$

$$t_1^{\mathrm{LF}} = 1 - t_2^{\mathrm{LF}}. \tag{SI 34}$$

Thus, if convection is negligible, the phenomenological parameter $\tau^{\mathrm{CMF}}$ describing the CMF-transport parameter of the first species, becomes the independent external transference number of the second species.

## I. Thermal Aspects

In this section, we focus on thermal aspects of our electrolyte transport theory. First, in section SI 1 I 1, we derive the missing transport equation for temperature ("heat equation"). Next, in section SI 1 I 2, we discuss transport phenomena which arise from temperature inhomogeneities. Finally, in section SI 1 I 3, we state our thermal model for the free energy density.

### *1. Heat Equation*

To account for thermal aspects, temperature is comprised in the materials law of the free energy density. However, when temperature is not set constant, an additional transport equation is mandatory. In this section, we close the set of transport equations by deriving the missing transport equation for temperature ("heat equation").

For this purpose, we take a step back to the entropy inequality (eq. (11)), which bears a somewhat hybrid function. Primarily, it served as motivation for the definition of the entropy production rate $\mathcal{R}$, and, up to now, was not made use of further. However, since we derived the thermodynamically consistent expression for $\mathcal{R}$ (eq. (47)), we can express the entropy inequality such that

it exhibits the form of a balance law (neglecting $h$),

$$\rho T\dot{s} = \mathcal{R} - T\nabla\boldsymbol{\xi}_s. \tag{SI 35}$$

Indeed, the set of transport equations, eqs. (67) to (70), and eq. (SI 35) suffice to describe the evolution of temperature, because the entropy density inherits it's material law from the free energy density via the constitutive equation 18,

$$\rho\dot{s}(T, c_\alpha, \mathbf{D}, \boldsymbol{\kappa}) = \rho\frac{\partial s}{\partial T}\cdot\dot{T} + \rho\sum_{\beta=1}^{\mathrm{N}}\frac{\partial s}{\partial c_\beta}\cdot\dot{c}_\beta + \rho\frac{\partial s}{\partial \mathbf{D}}\cdot\dot{\mathbf{D}} + \rho\frac{\partial s}{\partial \boldsymbol{\kappa}} : \dot{\boldsymbol{\kappa}}. \tag{SI 36}$$

We solve this equation for $\dot{T}$, substitute eq. (SI 35) and use the definition for the heat capacity, $\mathcal{C} = \rho T\cdot\partial s/\partial T$, given in the main text. Thus,

$$\mathcal{C}\dot{T} = \mathcal{R} - T\nabla\boldsymbol{\xi}_s - \rho T\sum_{\beta=1}^{\mathrm{N}}\frac{\partial s}{\partial c_\beta}\cdot\dot{c}_\beta - \rho T\frac{\partial s}{\partial \mathbf{D}}\cdot\dot{\mathbf{D}} - \rho T\frac{\partial s}{\partial \boldsymbol{\kappa}} : \dot{\boldsymbol{\kappa}}. \tag{SI 37}$$

Next, we transfer the derivatives of the entropy density in eq. (SI 37) to flux-terms using eq. (18), $\partial s/\partial \Upsilon_A = -\partial/\partial T\cdot\partial\varphi_{\mathrm{H}}/\partial\Upsilon_A$. These derivatives can be evaluated using eqs. (19) to (21) (note that all primary variables are independent, $\partial\Upsilon_A/\partial T|_{\Upsilon_A\neq T} = 0$), and using the equation of motion for the concentrations eq. (5),

$$\mathcal{C}\dot{T} = \mathcal{R} - T\nabla\boldsymbol{\xi}_s + T\frac{\partial}{\partial T}\left(\rho\varphi_{\mathrm{H}} - \sum_{\alpha=1}^{\mathrm{N}} c_\alpha\mu_\alpha\right)\cdot\nabla\mathbf{v} + \frac{\partial\mathbf{E}}{\partial T}\cdot\dot{\mathbf{D}} - T\sum_{\alpha=1}^{\mathrm{N}}\nabla\mathbf{N}_\alpha\cdot\frac{\partial\mu_\alpha}{\partial T}. \tag{SI 38}$$

The quantitiy $p^{el} = \rho\varphi_{\mathrm{H}} - \sum_{\alpha=1}^{\mathrm{N}} c_\alpha\mu_\alpha$ appearing in the third term on the right hand side is often used as definition for the elastic pressure.[16,17] Usually, a temperature-dependence of the material parameters (*e.g.*, viscosity coefficients) is neglected, such that $(\partial_T p^{el})\cdot\nabla\mathbf{v} = (\partial_T p)\cdot\nabla\mathbf{v}$, where $p = -\,\mathrm{tr}(\boldsymbol{\sigma})/3$ is the mean normal stress. In a linear dielectric model, $\mathbf{E} = (1+\chi)\mathbf{D}$, the fourth term on the right side becomes $\mathbf{D}\cdot\partial\chi/\partial T\cdot\dot{\mathbf{D}}$. Thus, this term vanishes when the temperature dependence of the susceptibility is neglected.[14] Furthermore, eq. (SI 38) contains redundant fluxes as the sum appearing in the last term on the right side begins with $\alpha = 1$. By substitution of eq. (70) and eq. (28), we reduce to the independent set of N-1 fluxes,

$$\mathcal{C}\dot{T} = \mathcal{R} - T\nabla\boldsymbol{\xi}_s - T\frac{\partial\left(\tilde{\mu}_2 + \tilde{\nu}_2 p\right)}{\partial T}\cdot\frac{1}{F\tilde{z}_2}\nabla\mathcal{J} - T\sum_{\alpha=3}^{\mathrm{N}}\frac{\partial(\tilde{\tilde{\mu}}_\alpha + \tilde{\tilde{\nu}}_\alpha p)}{\partial T}\cdot\nabla\mathbf{N}_\alpha + \frac{\partial\mathbf{E}}{\partial T}\cdot\dot{\mathbf{D}}. \tag{SI 39}$$

where $\mathcal{R}$ is determined by eq. (47).

*2. Hydrodynamical Expansion*

To obtain a better understanding of the mixing-term appearing in the entropy inequality eq. (47), we define the vector of N-1 thermodynamic diffusion-fluxes $\Psi_{\text{red}}$ and the vector of N-1 thermodynamic forces $\mathcal{X}_{\text{red}}$,

$$\Psi_{\text{red}} = (\mathbf{N}_3 - t_3\mathcal{J}/F\tilde{z}_3\ , \dots , \mathbf{N}_{\text{N}} - t_{\text{N}}\mathcal{J}/F\tilde{z}_{\text{N}}\ , \boldsymbol{\xi}_s - \beta\mathcal{J})^T, \tag{SI 40}$$

$$\mathcal{X}_{\text{red}} = (\boldsymbol{\nabla}\tilde{\tilde{\mu}}_3, \dots , \boldsymbol{\nabla}\tilde{\tilde{\mu}}_{\text{N}}, \boldsymbol{\nabla}T)^T. \tag{SI 41}$$

Both are related by the N-1×N-1 semi-positive definite diffusion-matrix $\mathcal{D}_{\text{red}} = (\mathcal{D}_{(\alpha)(\beta)})|_{\alpha,\beta\geq 3}$, such that the transport eqs. (43) and (44), and the entropy inequality become,

$$\Psi_{\text{red}} = -\mathcal{D}_{\text{red}} \cdot \mathcal{X}_{\text{red}}, \tag{SI 42}$$

$$\mathcal{R} = \boldsymbol{\tau} : \boldsymbol{\kappa} + \mathcal{J}^2\Big/\kappa + \mathcal{X}_{\text{red}}^T \cdot \mathcal{D}_{\text{red}} \cdot \mathcal{X}_{\text{red}} \geq 0. \tag{SI 43}$$

The chemical potentials $\tilde{\tilde{\mu}}_\alpha(\boldsymbol{\Upsilon})$ inherit the variable set $\boldsymbol{\Upsilon} = (T, \{c_\beta\}, \mathbf{D}, \boldsymbol{\kappa})$ from the free energy via the constitutive equation eq. (18). In particular, using the chain-law,

$$\boldsymbol{\nabla}\mu_\alpha = \frac{\partial}{\partial c_\alpha}\sum_A \frac{\partial(\rho\varphi_{\text{H}})}{\partial \Upsilon_A}\cdot\boldsymbol{\nabla}\Upsilon_A = \underbrace{\frac{\partial\mathbf{E}}{\partial c_\alpha}}_{\frac{\partial\mu_\alpha}{\partial\mathbf{D}}}\cdot\varrho + \sum_\beta \frac{\partial\mu_\alpha}{\partial c_\beta}\cdot\boldsymbol{\nabla}c_\beta - \underbrace{\frac{\partial(\rho s)}{\partial c_\alpha}}_{-\frac{\partial\mu_\alpha}{\partial T}}\cdot\boldsymbol{\nabla}T. \tag{SI 44}$$

In a linear dielectric medium, where $\mathbf{E} = (1+\chi)\mathbf{D}$, we get $\partial\mu_\alpha/\partial\mathbf{D} = \mathbf{D}\cdot\partial\chi/\partial c_\alpha$. In this case, $\partial\chi/\partial c_\alpha$ determines if the chemical potential depends on the electric field $\mathbf{D}$. For example, in ion-conducting solid-electrolytes, the polarizability of the electrolyte depends on ion-concentration. However, such contributions are usually neglected in liquid electrolytes.[14] Thus, we set $\partial\mathbf{E}/\partial T = 0$, and $\boldsymbol{\nabla}\mu_\alpha$ can be expanded in derivatives with respect to concentrations and temperature alone.

Thus, we can expand the thermodynamic forces, which are determined by the gradients of the chemical potentials and temperature, alternatively in the gradients of the concentrations and temperature, via

$$\mathcal{X}_{\text{red}} = \begin{pmatrix} \frac{\partial\tilde{\tilde{\mu}}_3}{\partial c_1} & \dots & \frac{\partial\tilde{\tilde{\mu}}_3}{\partial c_{\text{N}}} & \frac{\partial\tilde{\tilde{\mu}}_3}{\partial T} \\ \vdots & \ddots & \vdots & \vdots \\ \frac{\partial\tilde{\tilde{\mu}}_{\text{N}}}{\partial c_1} & \dots & \frac{\partial\tilde{\tilde{\mu}}_{\text{N}}}{\partial c_{\text{N}}} & \frac{\partial\tilde{\tilde{\mu}}_{\text{N}}}{\partial T} \\ 0 & \dots & 0 & 1 \end{pmatrix}\cdot\begin{pmatrix} \boldsymbol{\nabla}c_1 \\ \vdots \\ \vdots \\ \boldsymbol{\nabla}c_{\text{N}} \\ \boldsymbol{\nabla}T \end{pmatrix}. \tag{SI 45}$$

However, due to the expansion (62), the independent forces appearing on the right side of eq. (SI 45) are given by the vector of N forces, defined by

$$\mathcal{Z} = (\nabla\varrho/F\ , \nabla c_3, \ldots, \nabla c_{\mathrm{N}}, \nabla T)^T. \tag{SI 46}$$

However, a (N+1)×N matrix $\mathcal{M}(\nu_\alpha, M_\alpha)$ exists (see section SI 1 J), which relates both sets of variables,

$$(\nabla c_1, \ldots, \nabla c_{\mathrm{N}}, \nabla T)^T = \mathcal{M} \cdot \mathcal{Z}. \tag{SI 47}$$

We substitute this relation into eq. (SI 45), which suggests the definition of a (N−1) × N matrix $\boldsymbol{\mathit{đ}}$, such that

$$\mathcal{X}_{\mathrm{red}} = \boldsymbol{\mathit{đ}} \cdot \mathcal{Z}, \tag{SI 48}$$

where

$$\begin{pmatrix} đ_{3\varrho} & đ_{33} & \ldots & đ_{3\mathrm{N}} & \partial_T\tilde{\tilde{\mu}}_3 \\ \vdots & \vdots & \ddots & \vdots & \vdots \\ đ_{\mathrm{N}\varrho} & đ_{\mathrm{N}3} & \ldots & đ_{\mathrm{NN}} & \partial_T\tilde{\tilde{\mu}}_{\mathrm{N}} \\ 0 & 0 & \ldots & 0 & 1 \end{pmatrix} = \begin{pmatrix} \frac{\partial\tilde{\tilde{\mu}}_3}{\partial c_1} & \cdots & \frac{\partial\tilde{\tilde{\mu}}_3}{\partial c_{\mathrm{N}}} & \frac{\partial\tilde{\tilde{\mu}}_3}{\partial T} \\ \vdots & \ddots & \vdots & \vdots \\ \frac{\partial\tilde{\tilde{\mu}}_{\mathrm{N}}}{\partial c_1} & \cdots & \frac{\partial\tilde{\tilde{\mu}}_{\mathrm{N}}}{\partial c_{\mathrm{N}}} & \frac{\partial\tilde{\tilde{\mu}}_{\mathrm{N}}}{\partial T} \\ 0 & \ldots & 0 & 1 \end{pmatrix} \cdot \mathcal{M}. \tag{SI 49}$$

Here, we use a special notation defined as follows. Greek indices denote independent species, *viz.* $3 \leq \alpha \leq \mathrm{N}$, where $\alpha \neq T$ and $\alpha \neq \varrho$. The index "$\varrho$" relates to the first non-vanishing independent force $\nabla\varrho/F$, whereas the index "$T$" relates to the independent force $\nabla T$.

Using eq. (SI 42) suggests the definition of the (N−1) × N hydrodynamical expansion matrix $\boldsymbol{Đ} = \mathcal{D}_{\mathrm{red}} \cdot \boldsymbol{\mathit{đ}}$, such that

$$\Psi_{\mathrm{red}} = -\boldsymbol{Đ} \cdot \mathcal{Z}, \tag{SI 50}$$

where

$$\boldsymbol{Đ} = \begin{pmatrix} Đ_{3\varrho} & Đ_{33} & \ldots & Đ_{3\mathrm{N}} & \mathsf{S}_3 \\ \vdots & \vdots & \vdots & \vdots & \vdots \\ \vdots & \vdots & \vdots & \vdots & \vdots \\ Đ_{\mathrm{N}\varrho} & Đ_{\mathrm{N}3} & \ldots & Đ_{\mathrm{NN}} & \mathsf{S}_{\mathrm{N}} \\ \mathsf{D}_\varrho & \mathsf{D}_3 & \ldots & \mathsf{D}_{\mathrm{N}} & \lambda \end{pmatrix}. \tag{SI 51}$$

| Term | Name | Effect |
|---|---|---|
| $S_\alpha = \mathcal{D}_{\alpha T} + \sum_{\gamma=1}^{N} \mathcal{D}_{\alpha\gamma} \cdot \boldsymbol{đ}_{\gamma T} \cdot \partial\tilde{\tilde{\mu}}_\gamma/\partial T$ | Soret coefficients. | Thermophoresis. |
| $\breve{\beta} = \beta + \sum_{\beta=3}^{N} t_\beta/F^2\tilde{z}_\beta \cdot \partial\tilde{\tilde{\mu}}_\beta/\partial T$ | Seebeck coefficient. | Thermophoresis. |
| $D_\alpha = Đ_{\alpha T}$ | Dufour coefficients. | "Inverse" thermophoresis. |
| $D_\varrho = Đ_{\varrho T}$ | Dufour coefficient. | Double-layer effect. |
| $\lambda = Đ_{TT} = \gamma/T - \beta^2\kappa + \sum_{\gamma=3}^{N} \mathcal{D}_{T\gamma} \cdot \partial\tilde{\tilde{\mu}}_\gamma/\partial T$ | Heat conductivity. | Thermal conduction. |

TABLE SI 1. Hydrodynamical thermal coefficients.

All thermal coefficients $S_\alpha$, $D_\alpha$ and $\lambda$ of $\boldsymbol{Đ}$ are defined in table SI 1, and will be motivated below. Note that the definition of $\boldsymbol{Đ} = \mathcal{D}_{\text{red}} \cdot \boldsymbol{đ}$ is subject to the rule that it acts on $\mathcal{Z}$ according to $\boldsymbol{Đ}\mathcal{Z} = \mathcal{D}_{\text{red}} \cdot (\boldsymbol{đ}\mathcal{Z})$.

In order to express the mixing term in eq. (SI 43) using the independent forces $\mathcal{Z}$, we define the N×N *hydrodynamical diffusion matrix* $\boldsymbol{H}$, by

$$\boldsymbol{H} = \boldsymbol{Đ}^T \boldsymbol{đ} \tag{SI 52}$$

such that

$$\mathcal{R} = \boldsymbol{\tau} : \boldsymbol{\kappa} + \mathcal{J}^2\big/\kappa + \mathcal{Z}^T \cdot \boldsymbol{H} \cdot \mathcal{Z}. \tag{SI 53}$$

**Lemma 2** *The* N×N *hydrodynamic diffusion matrix* $\boldsymbol{H}$ *is symmetric and semi-positive definite.*

This can be seen as follows. By construction, $\boldsymbol{H}^T = \boldsymbol{đ}^T\boldsymbol{Đ} = \boldsymbol{đ}^T\mathcal{D}_{\text{red}}\boldsymbol{đ} = (\mathcal{D}_{\text{red}}^T\boldsymbol{đ})^T\boldsymbol{đ} = \boldsymbol{H}$. Furthermore, the mixing part in the entropy inequality is $\mathcal{Z}^T\boldsymbol{H}^T\mathcal{Z} = \mathcal{X}_{\text{red}}^T\mathcal{D}_{\text{red}}\mathcal{X}_{\text{red}} \geq 0$. Thus, due to symmetry, $\boldsymbol{H}$ is semi-positive definite.

The hydrodynamical matrix $\boldsymbol{Đ}$ comprises various thermal effects. These can be evaluated by expanding the thermodynamic fluxes $\Psi_{\text{red}}$ in the independent forces $\mathcal{Z}$, as described by eq. (SI 50),

$$\mathbf{N}_\alpha - \frac{t_\alpha}{F\tilde{z}_\alpha}\mathcal{J} = -\frac{1}{F}Đ_{\alpha\varrho} \cdot \boldsymbol{\nabla}\varrho - \sum_{\beta=3}^{N} Đ_{\alpha\beta} \cdot \boldsymbol{\nabla}c_\beta - S_\alpha \cdot \boldsymbol{\nabla}T, \tag{SI 54}$$

$$\boldsymbol{\xi}_s - \beta\mathcal{J} = -\frac{1}{F}D_\varrho \cdot \boldsymbol{\nabla}\varrho - \sum_{\beta=3}^{N} D_\beta \cdot \boldsymbol{\nabla}c_\beta - \lambda \cdot \boldsymbol{\nabla}T, \tag{SI 55}$$

$$\mathcal{J} = -\kappa\nabla\varphi - \frac{\kappa}{F^2}\sum_{\beta=3}^{\mathrm{N}}\frac{t_\beta}{F\tilde{z}_\beta}\text{đ}_{\beta\varrho}\cdot\nabla\varrho - \frac{\kappa}{F}\sum_{\gamma,\beta=3}^{\mathrm{N}}\frac{t_\beta\text{đ}_{\beta\gamma}}{F\tilde{z}_\beta}\cdot\nabla c_\gamma - \kappa\breve{\beta}\cdot\nabla T. \qquad \text{(SI 56)}$$

Thermophoresis ("Ludwig-Soret-effect") describes fluxes of mass and charge due to temperature gradients. It is measured by the Soret coefficients $S_\alpha$, and the thermophoretic Seebeck coefficient $\breve{\beta}$. The "inverse"-Soret effect measures flux of heat due to concentration-gradients, or gradients in $\varrho$. It is measured by the Dufour-coefficients $D_\alpha, D_\varrho$. However, electrolytes can safely be assumed electroneutral in the bulk electrolyte.[14] It is only in confined regions, *e.g.* the electrochemical double-layer, where $\varrho \neq 0$. Thus, $D_\varrho$ measures a thermal double-layer contribution. Furthermore, $\lambda = Đ_{TT}$ defines the hydrodynamical heat conductivity. We collect all definitions in table SI 1.

To study the influence of these thermal phenomena on temperature, we express the heat equation using the independent forces $\mathcal{Z}$. For this purpose, we substitute eqs. (SI 54) and (SI 55) into eq. (SI 39). Furthermore, we assume that temperature inhomogeneities in the chemical potentials and the pressure are equilibrated very fast. Hence, we neglect the terms $\nabla[\partial_T(\tilde{\mu}_2 + \tilde{\nu}_2 p)]$ and $\nabla[\partial_T(\tilde{\tilde{\mu}}_\alpha + \tilde{\tilde{\nu}}_\alpha p)]$. From the definition in eq. (37) it follows that $\nabla\beta = -\beta\nabla\log\kappa + F/\kappa\cdot\sum_{\alpha=2}^{\mathrm{N}}\nabla\mathcal{L}_{\alpha T}\cdot\tilde{z}_\alpha$. In this expression, we neglect the logarithmic term and assume that the only term depending on temperature is $\mathcal{L}_{\alpha T}(T)$, hence $\nabla\beta(T) = \partial\beta/\partial T\cdot\nabla T$. Usually, the Thomson-relation $\mu_\mathrm{T} = T\cdot\partial\beta/\partial T$, is used in the heat equation.[14] Here, $\mu_\mathrm{T} = F/\kappa T\cdot\sum_{\alpha=2}^{\mathrm{N}}\partial_T\mathcal{L}_{\alpha T}\tilde{z}_\alpha$. Therefore, the hydrodynamical expansion of the heat equation becomes

$$\begin{aligned} C\dot{T} =& \mathcal{R} - \mu_\mathrm{T}\mathcal{J}\nabla T - T\left[\beta + \frac{\partial}{\partial T}\left(\frac{\tilde{\mu}_2 + \tilde{\nu}_2 p}{F\tilde{z}_2} + \sum_{\alpha=3}^{\mathrm{N}} t_\alpha\frac{\tilde{\tilde{\mu}}_\alpha + \tilde{\tilde{\nu}}_\alpha p}{F\tilde{z}_\alpha}\right)\right]\nabla\mathcal{J} \\ &+ \frac{T}{F}\nabla\left[\left(D_\varrho + \sum_{\alpha=3}^{\mathrm{N}}\frac{\partial\left(\tilde{\tilde{\mu}}_\alpha + \tilde{\tilde{\nu}}_\alpha p\right)}{\partial T}\cdot Đ_{\alpha\varrho}\right)\nabla\varrho\right] \\ &+ T\sum_{\gamma=3}^{\mathrm{N}}\nabla\left[\left(D_\gamma + \sum_{\alpha=3}^{\mathrm{N}}\frac{\partial\left(\tilde{\tilde{\mu}}_\alpha + \tilde{\tilde{\nu}}_\alpha p\right)}{\partial T}\cdot Đ_{\alpha\gamma}\right)\nabla c_\gamma\right] \\ &+ T\nabla\left[\left(\lambda + \sum_{\alpha=3}^{\mathrm{N}}\frac{\partial\left(\tilde{\tilde{\mu}}_\alpha + \tilde{\tilde{\nu}}_\alpha p\right)}{\partial T}\cdot S_\alpha\right)\nabla T\right]. \end{aligned} \qquad \text{(SI 57)}$$

Thus, the hydrodynamical thermal coefficients $\beta, D_\varrho, D_\gamma, \lambda$ experience corrections stemming from the derivatives $\partial s/\partial c_\gamma$. These corrections take account for temperature-inhomogeneities of the chemical potentials and pressure. This suggests the following definitions.

$$\beta^p = \tilde{\beta} + \frac{1}{F\tilde{z}_2}\frac{\partial(\tilde{\nu}_2 p)}{\partial T} + \sum_{\alpha=3}^{\mathrm{N}}\frac{t_\alpha}{F\tilde{z}_\alpha}\frac{\partial(\tilde{\tilde{\nu}}_\alpha p^{\mathrm{td}})}{\partial T}, \quad \text{where} \quad \tilde{\beta} = \breve{\beta} + \frac{1}{F\tilde{z}_2}\frac{\partial\tilde{\mu}_2}{\partial T}, \qquad \text{(SI 58)}$$

$$\tilde{D}^p_\varrho = \tilde{D}_\varrho + \sum_{\alpha=3}^{\mathrm{N}} Đ_{\alpha\varrho} \cdot \frac{\partial(\tilde{\tilde{\nu}}_\alpha p^{\mathrm{td}})}{\partial T}, \quad \text{where} \quad \tilde{D}_\varrho = D_\varrho + \sum_{\alpha=3}^{\mathrm{N}} Đ_{\alpha\varrho} \cdot \frac{\partial \tilde{\tilde{\mu}}_\alpha}{\partial T}, \tag{SI 59}$$

$$\tilde{D}^p_\gamma = \tilde{D}_\gamma + \sum_{\alpha=3}^{\mathrm{N}} Đ_{\alpha\gamma} \cdot \frac{\partial(\tilde{\tilde{\nu}}_\alpha p^{\mathrm{td}})}{\partial T}, \quad \text{where} \quad \tilde{D}_\gamma = D_\gamma + \sum_{\alpha=3}^{\mathrm{N}} Đ_{\alpha\gamma} \cdot \frac{\partial \tilde{\tilde{\mu}}_\alpha}{\partial T}, \tag{SI 60}$$

$$\tilde{\lambda}^p = \tilde{\lambda} + \sum_{\alpha=3}^{\mathrm{N}} S_\alpha \cdot \frac{\partial\left(\tilde{\tilde{\nu}}_\alpha p^{\mathrm{td}}\right)}{\partial T}, \quad \text{where} \quad \tilde{\lambda} = \lambda + \sum_{\alpha=3}^{\mathrm{N}} S_\alpha \cdot \frac{\partial \tilde{\tilde{\mu}}_\alpha}{\partial T}. \tag{SI 61}$$

The hydrodynamical heat equations eq. (SI 57) thus becomes,

$$C\dot{T} = \boldsymbol{\tau} : \boldsymbol{\kappa} + \frac{\mathcal{J}^2}{\kappa} + \mathcal{Z}^T \boldsymbol{H} \mathcal{Z} - \mu_{\mathrm{T}} \mathcal{J} \nabla T - T \tilde{\beta}^p \nabla \mathcal{J} + \frac{T}{F} \nabla \tilde{D}^p_\varrho \nabla \varrho + T \sum_{\gamma=3}^{\mathrm{N}} \nabla \tilde{D}^p_\gamma \nabla c_\gamma + T \nabla \tilde{\lambda}^p \nabla T. \tag{SI 62}$$

We observe various heating effects. Strictly positive contributions, thus increasing temperature, are mechanical stress / viscous friction, Joule heating (first and second term), and entropy of mixing (third term). The Thomson effect (fourth term) comprises heat-transport along electric currents $\mathcal{J}$, which either decrease or increase temperature. The fifth and sixth term describe thermo-migration and thermo-charging. Both vanish in electroneutral regions (bulk electrolyte). The seventh term is the Dufour-effect, which implies temperature variations due to species-diffusion. The last term describes thermal conduction.

Lemma 2 implies constraints on the coefficients of $\boldsymbol{H}$. Writing out the the mixing term appearing in the entropy inequality, eq. (SI 53), explicitely,

$$\mathcal{Z}^T \cdot \boldsymbol{H} \cdot \mathcal{Z} = \frac{1}{F^2} H_{\varrho\varrho} (\nabla\varrho)^2 + \sum_{\alpha,\beta=3}^{\mathrm{N}} H_{\alpha\beta} (\nabla c_\alpha)(\nabla c_\beta) + 2 \sum_{\alpha=3}^{\mathrm{N}} \mathcal{H}_{T\alpha} (\nabla c_\alpha)(\nabla T) + 2 H_{T\varrho} (\nabla\varrho)(\nabla T)$$
$$+ 2 H_{\alpha\varrho} (\nabla\varrho)(\nabla c_\alpha) + H_{TT} (\nabla T)^2 \geq 0. \tag{SI 63}$$

Thus, all diagonal elements $H_{\varrho\varrho}$, $H_{\alpha\alpha}$, $H_{TT}$ are non-negative, and the submatrix $H_{\alpha\beta}$ is semi-positive definite. Note that

$$H_{TT} = \lambda + \sum_{\gamma=3}^{\mathrm{N}} S_\gamma \cdot \frac{\partial \tilde{\tilde{\mu}}_\gamma}{\partial T} = \tilde{\lambda}^p - \sum_{\gamma=3}^{\mathrm{N}} S_\gamma \cdot \frac{\partial\left(\tilde{\tilde{\nu}}_\gamma p^{\mathrm{td}}\right)}{\partial T} \geq 0. \tag{SI 64}$$

Thus, $\tilde{\lambda}^p \geq 0$, if the partial molar volumes and the pressure do not depend on temperature. In this case, heat conduction (last term in eq. (SI 62)) equilibrates temperature inhomogeneities.

### 3. *Thermal Model for the Free Energy Density*

Yet, the mixing term, $RT \sum_{\alpha=1}^{\mathrm{N}} c_\alpha \ln(c_\alpha/c)$, and the interaction free energy determine the temperature dependence of our model free energy (eq. (52)). For simplicity, we neglect $\rho\varphi^{\mathrm{int}}_{\mathrm{H}}$ in this

| Term | Effect | Interpretation |
|---|---|---|
| $\boldsymbol{\tau} : \boldsymbol{\kappa} \geq 0$ | Viscous friction. | Increases temperature. |
| $\mathcal{J}^2/\kappa \geq 0$ | Joule heating | Increases temperature. |
| $-\mu_\mathrm{T}\mathcal{J}\boldsymbol{\nabla}T$ | Thomson effect. | Thermoelectric effect. |
| $\mathcal{Z}^T \cdot \boldsymbol{H} \cdot \mathcal{Z}$ | Multi-component heat of mixing. | Increases temperature. |
| $-T\tilde{\beta}^p\boldsymbol{\nabla}\mathcal{J} + T/F \cdot \boldsymbol{\nabla}\tilde{D}^p_\varrho\boldsymbol{\nabla}\varrho$ | Dufour-effect for charged systems. | Vanishes in electroneutral case. |
| $T\boldsymbol{\nabla}\sum_{\gamma=3}^{\mathrm{N}}\tilde{D}^p_\gamma\boldsymbol{\nabla}c_\gamma$ | Dufour-effect. | Species diffusion. |
| $T\boldsymbol{\nabla}(\tilde{\lambda}^p \cdot \boldsymbol{\nabla}T)$ | Thermal conduction. | Equilibrates temperature. |

TABLE SI 2. Contributions to the heat equation.

discussion.

Since the mixing term is linear in $T$, the internal energy density as well as the entropy density,

$$\rho u = -T^2 \cdot \frac{\partial}{\partial T}\left(\frac{\rho\varphi_\mathrm{H}}{T}\right), \quad \text{and} \quad \rho s = -\frac{\partial}{\partial T}\left(\rho\varphi_\mathrm{H}\right), \tag{SI 65}$$

do not depend on temperature at all. This clearly is in contradiction with experimental observations. Thus, we must extend our model by a thermal term.

For dilute electrolytes ($f_\alpha = 1$), we state our model for the thermal entropy,

$$\rho s_{th} = \ln(T/T_\mathrm{R}) \cdot \sum_{\alpha=1}^{\mathrm{N}} \rho_\alpha C_\alpha, \tag{SI 66}$$

relative to a reference temperature $T_\mathrm{R}$. This simple model satisfies the requirements that it, (i), vanishes for constant temperature ($T = T_\mathrm{R}$), (ii), is strictly positive, and, (iii), increases for cooling and heating relative to the reference-temperature $T_\mathrm{R}$. Upon application of the constitutive equation for $s$ (eq. (18)), this model implies a thermal contribution to the free energy density,

$$\rho\varphi_\mathrm{H}^\mathrm{th} = (T - T_\mathrm{R} - T\ln T/T_\mathrm{R})\sum_{\alpha=1}^{\mathrm{N}} C_\alpha\rho_\alpha. \tag{SI 67}$$

This result equals the thermal model described by Guhlke.[12]

### J. Matrix Formulation of the Transport Theory

Let us first fresh up the notation introduced so-far, and introduce some more quantities. Depending on the context, we use different vectors comprising thermodynamic forces,

$$\mathcal{X}^T = (\nabla\mu_1, \ldots, \nabla\mu_N, \nabla T), \tag{SI 68}$$

$$\tilde{\mathcal{X}}^T = (\nabla\tilde{\mu}_2, \ldots, \nabla\tilde{\mu}_N, \nabla T), \tag{SI 69}$$

$$\mathcal{X}^T_{\text{red}} = (\nabla\tilde{\tilde{\mu}}_3, \ldots, \nabla\tilde{\tilde{\mu}}_N, \nabla T), \tag{SI 70}$$

and different vectors comprising thermodynamic fluxes,

$$\psi^T = (\mathbf{N}_2, \ldots, \mathbf{N}_N, \boldsymbol{\xi}_s), \tag{SI 71}$$

$$\psi^T_{\text{red}} = (\mathbf{N}_3, \ldots, \mathbf{N}_N, \boldsymbol{\xi}_s). \tag{SI 72}$$

Furthermore, we introduce two vectors of reduced quantities and two vectors comprising weighted transport coefficients,

$$\tilde{\boldsymbol{z}} = (\tilde{z}_2, \ldots, \tilde{z}_N)^T, \tag{SI 73}$$

$$\tilde{\mathbf{v}} = (\tilde{v}_2, \ldots, \tilde{v}_N)^T, \tag{SI 74}$$

$$\mathfrak{T}^T = (t_2/F\tilde{z}_2, \ldots, t_N/F\tilde{z}_N, \beta), \tag{SI 75}$$

$$\mathfrak{T}^T_{\text{red}} = (t_3/F\tilde{z}_3, \ldots, t_N/F\tilde{z}_N, \beta). \tag{SI 76}$$

There are two pricipal forms for a matrix-formulation of the transport equations. *Either*, we expand the thermodynamic forces in the independent forces, $\mathcal{X}_{\text{red}} = \boldsymbol{đ} \cdot \mathcal{Z}$, where the matrix $\boldsymbol{đ}$ comprises derivatives $\partial\tilde{\tilde{\mu}}_\alpha/c_\beta$ with $1 \leq \beta \leq$ N (see section SI 1 I 2). This expansion has the advantage that it illustrates how the transport equations depend on the concentration gradients. We evaluated this approach component-wise in eqs. (SI 54) to (SI 56). However, the derivatives comprised in $\boldsymbol{đ}$ are hardly accessible.

*Alternatively*, we do not evaluate the gradients $\nabla\tilde{\tilde{\mu}}_\alpha$ according to their materials law, but first reduce to the set of all thermodynamic forces $\mathcal{X}$, and then evaluate the gradients $\nabla\mu_\alpha$.

In this section, we will follow the second approach. For this purpose, we introduce the N-1×N

valency-matrix $\mathcal{Z}$, and the N×N+1 mass-matrix $\mathfrak{M}$

$$\mathcal{Z}(z_\alpha, M_\alpha) = \left( \begin{bmatrix} -\tilde{z}_3/\tilde{z}_2 \\ \vdots \\ -\tilde{z}_N/\tilde{z}_2 \\ 0 \end{bmatrix} \begin{bmatrix} \ddots & & \\ & \mathrm{diag}^{[(N-1)\times(N-1)]}(1) & \\ & & \ddots \end{bmatrix} \right), \tag{SI 77}$$

and

$$\mathfrak{M}(M_\alpha) = \left( \begin{bmatrix} -M_2/M_1 \\ \vdots \\ -M_N/M_1 \\ 0 \end{bmatrix} \begin{bmatrix} \ddots & & \\ & \mathrm{diag}^{[N\times N]}(1) & \\ & & \ddots \end{bmatrix} \right), \tag{SI 78}$$

where, $\mathrm{diag}^{[N\times N]}(1)$ denotes a quadratic N-dimesnional diagonal-matrix with equal entries 1.

With the help of these two matrices, the different set of potentials can be related via simple products,

$$(\tilde{\mu}_2, \ldots, \tilde{\mu}_N, T)^T = \mathfrak{M} \cdot (\mu_1, \ldots, \mu_N, T)^T, \tag{SI 79}$$

and

$$(\tilde{\tilde{\mu}}_3, \ldots, \tilde{\tilde{\mu}}_N, T)^T = \mathcal{Z} \cdot (\tilde{\mu}_2, \ldots, \tilde{\mu}_N, T)^T \tag{SI 80}$$

$$= \mathcal{Z} \cdot \mathfrak{M} \cdot (\mu_1, \ldots, \mu_N, T)^T. \tag{SI 81}$$

Since $\mathcal{Z}$ and $\mathfrak{M}$ are functions of constant material-parameters, this expansion can be transferred to the vectors of thermodynamic forces. In particular,

$$\mathcal{X}_{\mathrm{red}} = \mathcal{Z} \cdot \mathfrak{M} \cdot \mathcal{X}. \tag{SI 82}$$

The center-of-mass current $\mathcal{J}$ is determined by eq. (46). Substitution of the expansion eq. (SI 82) allows to express $\mathcal{J}$ using $\mathcal{X}$,

$$\mathcal{J} = -\kappa \cdot (\boldsymbol{\nabla}\Phi) - \kappa \cdot \mathfrak{T}^T \cdot \mathfrak{M} \cdot \mathcal{X} \tag{SI 83a}$$

$$= -\kappa \cdot \left(1,\ [\mathfrak{M}^T \cdot \mathfrak{T}]^T\right) \cdot \begin{pmatrix} \boldsymbol{\nabla}\Phi \\ [\mathcal{X}] \end{pmatrix} \tag{SI 83b}$$

The thermodynamic fluxes comprised by $\psi$ are determined by eqs. (43) and (44), whereas $\mathbf{N}_2$ is determined by $\mathcal{J} = \sum_{\alpha=2}^{N} F\tilde{z}_\alpha \mathbf{N}_\alpha$. In order to expand $\psi$ in the thermodynamic forces $\mathcal{X}$,

we introduce a special notation which multiplies a vector-valued quantity as a scalar on another vector, *e.g.*

$$\mathcal{J} \odot \mathfrak{T} = \begin{pmatrix} \mathcal{J} \cdot \mathfrak{T}_2 \\ \vdots \\ \mathcal{J} \cdot \mathfrak{T}_\mathrm{N} \\ \mathcal{J} \cdot \beta \end{pmatrix}. \tag{SI 84}$$

Using this notation, we get $\psi = \mathcal{J} \odot \mathfrak{T} - \mathcal{D} \cdot \mathcal{Z} \cdot \mathcal{X}_\mathrm{red}$. Apparently, since $\mathcal{J} \odot \mathfrak{T} = -\kappa(\nabla\Phi) \odot \mathfrak{T} - \kappa \cdot \mathfrak{T} \otimes \mathfrak{T} \cdot \tilde{\mathcal{X}}$, we cannot completely express $\psi$ via $\mathcal{X}_\mathrm{red}$. Thus, the two vectors of thermodynqamic fluxes expanded in all chemical potentials and temperature, read

$$\psi = -\kappa \cdot (\nabla\Phi) \odot \mathfrak{T} - (\mathcal{D} \cdot \mathcal{Z} + \kappa \cdot \mathfrak{T} \otimes \mathfrak{T}) \cdot \mathfrak{M} \cdot \mathcal{X}^T \tag{SI 85a}$$

$$= -\left( \begin{bmatrix} \vdots \\ \kappa \cdot \mathfrak{T} \\ \vdots \end{bmatrix} \begin{bmatrix} \ddots & & \\ & (\mathcal{D} \cdot \mathcal{Z} + \kappa \cdot \mathfrak{T} \otimes \mathfrak{T}) \cdot \mathfrak{M} & \\ & & \ddots \end{bmatrix} \right) \cdot \begin{pmatrix} \nabla\Phi \\ \begin{bmatrix} \mathcal{X} \end{bmatrix} \end{pmatrix}. \tag{SI 85b}$$

and

$$\psi_\mathrm{red} = -\kappa \cdot (\nabla\Phi) \odot \mathfrak{T}_\mathrm{red} - (\mathcal{D}_\mathrm{red}\mathcal{Z} + \kappa \cdot \mathfrak{T}_\mathrm{red} \otimes \mathfrak{T}) \cdot \mathfrak{M} \cdot \mathcal{X} \tag{SI 86a}$$

$$= -\left\{ \mathfrak{T}_\mathrm{red} \otimes \kappa \cdot \begin{pmatrix} 1 \\ \begin{bmatrix} \mathfrak{M}^T \cdot \mathfrak{T} \end{bmatrix} \end{pmatrix} + \left( \begin{bmatrix} 0 \\ \vdots \\ 0 \end{bmatrix} \begin{bmatrix} \ddots & & \\ & \mathcal{D} \cdot \mathcal{Z} \cdot \mathfrak{M} & \\ & & \ddots \end{bmatrix} \right) \right\} \cdot \begin{pmatrix} \nabla\Phi \\ \begin{bmatrix} \mathcal{X} \end{bmatrix} \end{pmatrix}. \tag{SI 86b}$$

Using eqs. (SI 83) and eqs. (SI 86) we can easily state the matrix-form of the convection-equation (see eq. (63)),

$$\nabla \mathbf{v} = -\left( [\ \tilde{\mathbf{v}}^T\ ], 0 \right) \cdot (\nabla \odot \psi) = -\left( \tilde{\mathrm{v}}_2/F\tilde{z}_2\ , \tilde{\tilde{\mathrm{v}}}_3, \ldots, \tilde{\tilde{\mathrm{v}}}_\mathrm{N}, 0 \right) \cdot \begin{pmatrix} \nabla \mathcal{J} \\ \nabla \odot \begin{bmatrix} \psi_\mathrm{red} \end{bmatrix} \end{pmatrix}. \tag{SI 87}$$

The expansion eqs. (SI 83), eqs. (SI 86), eqs. (SI 85) and eq. (SI 87), are subject to a specific form of the free energy, which determines the form of $\mathcal{X}$. However, we can assume that any such model is a function of species-concentrations. Thus, $\nabla\mu_\alpha(\Upsilon) = (\sum_A \partial\mu_\alpha/\partial\Upsilon_A \cdot \nabla)\Upsilon_A|_{\Upsilon_A \neq c_\gamma} + \sum_{\gamma=1}^{\mathrm{N}} \partial\mu_\alpha/\partial c_\gamma \cdot \nabla c_\gamma$, and the the expansion eq. (SI 82) is supplemented by the expansion of all concentrations via the independent variables, eq. (62). In particular, for any number N of species, there exists a N×N matrix $\mathcal{M}(z_\alpha, \nu_\alpha)$, such that

$$(c_1,\ \ldots,\ c_\mathrm{N})^T = \mathcal{M} \cdot (1/z_{[2}\nu_{1]}\ ,\ \varrho/F\ ,\ c_3,\ \ldots, c_\mathrm{N})^T\ , \tag{SI 88}$$

where

$$\mathcal{M}(z_\alpha, \nu_\alpha) = \frac{1}{z_{[2}\nu_{1]}} \left( \begin{bmatrix} z_2 z_{[2}\nu_{1]} & -\nu_2 \\ -z_1 z_{[2}\nu_{1]} & \nu_1 \\ 0 & 0 \\ \vdots & \vdots \\ 0 & 0 \end{bmatrix} \begin{bmatrix} \begin{bmatrix} z_{[3}\nu_{2]} & z_{[4}\nu_{2]} & \dots & z_{[N}\nu_{2]} \\ -z_{[3}\nu_{1]} & -z_{[4}\nu_{1]} & \dots & -z_{[N}\nu_{1]} \end{bmatrix} \\ \begin{bmatrix} \\ \mathrm{diag}^{(N-2)\times(N-2)}(z_{[2}\nu_{1]}) \\ \\ \end{bmatrix} \end{bmatrix} \right). \qquad \text{(SI 89)}$$

| Material Parameters | Transport Parameters | Thermodynamic Quantities |
|---|---|---|
| $\mathfrak{M}(M_\alpha)$ | $\mathcal{L}$ | $\mathcal{J}$ |
| $\mathcal{Z}(z_\alpha, M_\alpha)$ | $\kappa = F\tilde{z}^T \cdot \mathcal{L} \cdot F\tilde{z}$ | $\psi, \psi_{\mathrm{red}}$ |
| $\nu_\alpha, \tilde{\nu}_\alpha, \tilde{\tilde{\nu}}_\alpha$ | $\mathfrak{T} = 1/\kappa \cdot \mathcal{L} \cdot F\tilde{z}$ | $\mathcal{X}, \mathcal{X}_{\mathrm{red}}$ |
| $\tilde{z} = (\tilde{z}_2, \dots, \tilde{z}_N)$ | $\mathcal{D} = \mathcal{L} - \kappa \cdot \mathfrak{T} \otimes \mathfrak{T}$ | |
| $\mathcal{M}(z_\alpha, \nu_\alpha)$ | | |

TABLE SI 3. Summary of the parameters and thermodynamic quantities.

Finally, we state the matrix-form of the isothermal transport equations, subject to the model-dependent form of the chemical potentials. In this case, the thermal coefficients in the $\psi_{\mathrm{red}}$, $\mathfrak{T}$, $\mathcal{D}$, $\mathcal{Z}$, $\mathfrak{M}$ and $\mathcal{X}$ are ommitted, such that

$$\partial_t \varrho = -\nabla \left( \mathcal{J} + \varrho \mathbf{v} \right), \qquad \text{(SI 90)}$$

$$\left( \partial_t c_3, \ \dots, \ \partial_t c_N \right)^T = -\nabla \odot \psi_{\mathrm{red}} - \nabla \odot \left( \mathbf{v} \cdot c_3, \ \dots, \ \mathbf{v} \cdot c_N \right)^T, \qquad \text{(SI 91)}$$

where the concentrations of the designated species, $c_1$ and $c_2$, are determined by eq. (SI 88). The the center-of-mass current $\mathcal{J}$, and the vector of independent mass-fluxes $\psi_{\mathrm{red}}$ are determined by eqs. SI 83 and SI 86. The convection velocity is determined by eq. (SI 87), which must be supplemented by a reaction-term $\sum_{\alpha=1}^{N} \nu_\alpha \cdot r_\alpha$, if necessary (see eq. (61)). If thermal aspects shall be discussed, the set of transport equations must be extended by eq. (SI 62).

### 1. *Example: Quaternary, Electroneutral Electrolyte in Isothermal Case*

Since we neglect temperature variations, we can eliminate the last column in the matrices $\mathcal{Z}$ and $\mathfrak{M}$, and the last entry in $\mathcal{X}$ and $\mathfrak{T}$. Also, since we assume electroneutrality, we can omitt the

second row in $\boldsymbol{\mathcal{M}}$. Altogether,

$$\mathcal{Z} = \begin{pmatrix} -\tilde{z}_3/\tilde{z}_2 & 1 & 0 \\ -\tilde{z}_4/\tilde{z}_2 & 0 & 1 \end{pmatrix}, \tag{SI 92}$$

$$\mathcal{M} = \begin{pmatrix} -M_2/M_1 & 1 & 0 & 0 \\ -M_3/M_1 & 0 & 1 & 0 \\ -M_4/M_1 & 0 & 0 & 1 \end{pmatrix}, \tag{SI 93}$$

$$\boldsymbol{\mathcal{M}} = \frac{1}{z_{[2\vee 1]}} \begin{pmatrix} z_2 z_{[2\vee 1]} & z_{[3\vee 2]} & z_{[4\vee 2]} \\ -z_1 z_{[2\vee 1]} & -z_{[3\vee 1]} & -z_{[4\vee 1]} \\ 0 & z_{[2\vee 1]} & 0 \\ 0 & 0 & z_{[2\vee 1]} \end{pmatrix}, \tag{SI 94}$$

$$(c_1,\ c_2,\ c_3,\ c_4)^T = \boldsymbol{\mathcal{M}} \cdot (1/z_{[2\vee 1]}\ ,\ c_3,\ c_4) \tag{SI 95}$$

$$\mathcal{X}^T = (\boldsymbol{\nabla}\mu_1,\ \boldsymbol{\nabla}\mu_2,\ \boldsymbol{\nabla}\mu_3,\ \boldsymbol{\nabla}\mu_4)^T, \tag{SI 96}$$

$$\mathcal{L} = \begin{pmatrix} \mathcal{L}_{22} & \mathcal{L}_{23} & \mathcal{L}_{24} \\ \mathcal{L}_{23} & \mathcal{L}_{33} & \mathcal{L}_{34} \\ \mathcal{L}_{24} & \mathcal{L}_{34} & \mathcal{L}_{44} \end{pmatrix}. \tag{SI 97}$$

When we neglect interactions in our electrolyte model, we get for the thermodynamic forces in our electrolyte model eq. (52)

$$\mathcal{X} = -\varrho \cdot (\boldsymbol{\nabla}\Phi) \odot (\nu_1,\ \nu_2,\ \nu_3,\ \nu_4)^T + RT\boldsymbol{\nabla} \odot (\ln f_1 c_1,\ \ln f_2 c_2,\ \ln f_3 c_3,\ \ln f_4 c_4)^T. \tag{SI 98}$$

### K. Transformation of Reference Species

Due to mass conservation, we designate one species, usually the physical species assigned to the species-index $\alpha = 1$, relative to which we introduce reduced sets of valences $\tilde{z}_\alpha$, chemical potentials $\tilde{\mu}_\alpha$ and partial molar volumes $\tilde{\nu}_\alpha$.

Since the choice of the designated species is arbitrary, our formalism shall be invariant under changing the designated species.

In this section, we first generalize the notation introduced in the main part, in order to track the underlying choice of designated species. Next, we apply this notation to the matrix formulation introduced in section SI 1 J, and derive the transformation behaviour of the reduced sets of quantities mentioned above. Using mass conservation, we then derive the transformation behaviour

of the set of thermodynamic fluxes eq. (SI 71). From the exact transformation rules for the potentials and fluxes, we derive the transformation behaviour of the Onsager matrix $\mathcal{L}$, and of the transport parameters, which are function of $\mathcal{L}$. Finally, we apply this formalism to the different reference-frames discussed in the main text.

For the sake of this discussion, we introduce a new set of indices comprising capital latin letters, $A, B, C, \ldots$ which relate to a fixed sequence of physical species. In addition, we assume a bijective assignment between the physical species $A, B, C, \ldots$, and the species-indices $\alpha, \beta, \gamma, \ldots$

We derive the transformation rules by changing the designated species from $\alpha = 1$ to any other index $\alpha \neq 1$, by preserving the bijective mapping between the physical indices and the species indices. (Alternatively, we could rearrange the assignment between the physical species and the species-indices. Thereby, the designated species would still refer to $\alpha = 1$, but the physical species assigned to the first species-index would differ. However, such an approach obfuscates the main line of reasoning by an additional layer of transformations.)

In this section, we neglect thermal aspects and thus all quantities are understood to be reduced as explained in section SI 1 J.

### 1. *Transformation of Reduced Quantities*

The reduced set of valences defined by eq. (26) refers to the special case where the designated species is $\alpha = 1$. Here, we generalize this notation and define reduced sets of valences relative to any designated species $A$,

$$\tilde{z}_B^{(A)}|_{B\neq A} = z_B|_{B\neq A} - M_B/M_A \cdot z_A|_{B\neq A}. \quad \text{(SI 99)}$$

Thus, two sets of reduced valences ($\tilde{z}_B^{(A)}$) and ($\tilde{z}_D^{(C)}$), defined relative to different designated species $A$, and $C$ respectively, are related by

$$\tilde{z}_B^{(A)} = \tilde{z}_B^{(C)}|_{B\neq A,C} - M_B/M_A \cdot \tilde{z}_A^{(C)}|_{B\neq A,C} \quad \text{(SI 100)}$$

In more general terms, any two sets of reduced quantities defined relative to two distinct designated species $A$, and $C$ respectively, are related by transformations $\mathfrak{M}^{(A\to C)}$,

$$\tilde{\mathbf{z}}^{(A)} = \mathfrak{M}^{(C\to A)} \cdot \tilde{\mathbf{z}}^{(C)}, \quad \text{(SI 101)}$$

$$\tilde{\boldsymbol{\nu}}^{(A)} = \mathfrak{M}^{(C\to A)} \cdot \tilde{\boldsymbol{\nu}}^{(C)}, \quad \text{(SI 102)}$$

$$\tilde{\mathcal{X}}^{(A)} = \mathfrak{M}^{(C\to A)} \cdot \tilde{\mathcal{X}}^{(C)}, \quad \text{(SI 103)}$$

where the (N-1)×(N-1)- dimensional matrix-representation of the transformation $\mathfrak{M}^{(A\to C)}$ is

$$\mathcal{M}_{DB}^{(C\to A)}|_{\substack{D\neq C\\B\neq A}} = \delta_{DB}|_{\substack{D\neq C\\B\neq A}} - M_B/M_D \cdot \delta_{AD}|_{\substack{D\neq C\\B\neq A}}. \tag{SI 104}$$

Note that there is no sum over the index "$D$", appearing on the left side. Again, the mass-matrix defined by eq. (SI 78) represents the special case where the designated species is $\alpha = 1$, and is related to the transformation matrix $\mathfrak{M}^{(2\to 1)}$ by elimination of the second column. This will become apparent in section SI 1 K 4.

Equation (SI 104) implies that the trivial transformation is the neutral element, $\mathfrak{M}^{(A\to A)} = \mathbf{Id}$. Of course, the cyclic transformation $\mathfrak{M}^{(C\to A)} \circ \mathfrak{M}^{(A\to C)}$ shall yield the neutral transformation $\mathfrak{M}^{(C\to C)} \equiv \mathbf{Id}$. Indeed, by construction, $\sum_{B\neq A} \mathcal{M}_{DB}^{(C\to A)}|_{D\neq C} \cdot \mathcal{M}_{BE}^{(A\to C)}|_{D\neq C} = \delta_{DE}|_{E,D\neq C}$. Therefore,

$$\mathfrak{M}^{(C\to A)} = \left(\mathfrak{M}^{(A\to C)}\right)^{-1}. \tag{SI 105}$$

### 2. *Transformation of Mass Fluxes*

In this sectoin, we neglect thermal aspects. Thus, we reduce the vector of thermodynamic fluxes defined by eq. (SI 71) to $\psi^T = (\mathbf{N}_2, \ldots, \mathbf{N}_\mathrm{N})$. However, this vector is merely the special case which we shall denote by $\psi^{(1)}$, following the rationale explained in the previous section. Due to mass-conservation, $\sum_A M_A \cdot \mathbf{N}_A = 0$, only N-1 of the mass-fluxes are independent. Thus, we can recover the vector of all fluxes

$$\psi_{\mathrm{all}}^T = (\mathbf{N}_1, \ldots, \mathbf{N}_\mathrm{N}) \tag{SI 106}$$

from any given representation $\psi^{(A)}$. To keep track of the reference species, we denote this function by $\psi_{\mathrm{all}}^T = \psi_{\mathrm{all}}^{(A)}(\psi^{(A)})$. It has a representation in terms of

$$\psi_{\mathrm{all}}^{(A)}(\psi^{(A)}) = \mathfrak{M}^{(A\to \mathrm{N})} \cdot \psi^{(A)}, \quad \text{where} \quad \mathcal{M}_{BD}^{(A\to \mathrm{N})} = \delta_{BD} - M_D/M_A \cdot \delta_{BA}. \tag{SI 107}$$

Likewise, the inverse transformation, which calculates $\psi^{(A)}$ from the vector of all fluxes $\psi_{\mathrm{all}}$, is given by

$$\psi^{(A)} = \mathfrak{M}^{(\mathrm{N}\to A)} \cdot \psi_{\mathrm{all}}, \quad \text{where} \quad \mathcal{M}_{BD}^{(\mathrm{N}\to A)} = \delta_{BD} - \delta_{AD}. \tag{SI 108}$$

From eqs. (SI 107) and (SI 108) follows the transformation rule between independent sets of fluxes relative to different designated species $A$, and $C$ respectively, ,

$$\psi^{(C)}\left(\psi^{(A)}\right) = \left(\mathfrak{M}^{(C\to A)}\right)^T \cdot \psi^{(A)}, \tag{SI 109}$$

where

$$\left[(\mathcal{M}^{(C\to A)})^T\right]_{BD} = \delta_{BD} - M_D/M_B \cdot \delta_{BA}. \tag{SI 110}$$

Apparently, the fluxes transform inversely and conjugated (via the transposed representation-matrix), as compared to the reduced quantities $\tilde{z}^{(A)}$, $\tilde{\mathcal{X}}^{(A)}$ and $\tilde{\mathbf{v}}^{(A)}$. As we shall see, this form of the transformation matrices implies simple transformation-rules for the transport parameters (see section SI 1 K 3).

The representation matrices for the transformation between the set of all fluxes and the different sets of independent fluxes exhibit the property,

$$\mathcal{M}^{(A\to\mathrm{N})} \cdot (\mathcal{M}^{(A\to C)})^T = \mathcal{M}^{(C\to\mathrm{N})}. \tag{SI 111}$$

From this property follows that the set of all fluxes obtained from different representations is invariant under changing the designated species,

$$\psi^{(A)}_{\mathrm{all}} = \psi^{(C)}_{\mathrm{all}}. \tag{SI 112}$$

### 3. *Transformation of Onsager Matrix and Transport Parameters*

The Onsager matrix $\mathcal{L}$ defined by eq. (31) couples the fluxes $\psi^{(1)}$ with the reduced set of forces $\tilde{\mathcal{X}}^{(1)}$. Relative to any choice $A$ for the designated species, specific Onsager matrices $\mathcal{L}^{(A)}$ exist. As consequence, relative to this choice, different sets of transport parameters exist.

From the transformation rules of the fluxes and reduced potentials, eqs. (SI 103) and (SI 109), follow directly the transformation rule for the Onsager matrix $\mathcal{L}$,

$$\mathcal{L}^{(C)} = (\mathcal{M}^{(C\to A)})^T \cdot \mathcal{L}^{(A)} \cdot \mathcal{M}^{(C\to A)}. \tag{SI 113}$$

This determines the transformation rules of the transport parameters $\kappa^{(A)}$, $\mathcal{T}^{(A)}$ and $\mathcal{D}^{(A)}$, being functions of $\mathcal{L}^{(A)}$.

eq. (36) represents the definition of the electric conductivity relative to the designated species $\alpha = 1$, $\kappa^{(1)}/F^2 = (\tilde{z}^{(1)})^T \cdot \mathcal{L}^{(1)} \cdot \tilde{z}^{(1)}$. We generalize this definition to any designated species $A$, which implies that

$$\kappa^{(A)} = F^2 \cdot (\tilde{z}^{(A)})^T \cdot \mathcal{L}^{(A)} \cdot \tilde{z}^{(A)} \tag{SI 114a}$$

$$= F^2 \cdot (\mathcal{M}^{(C\to A)} \cdot \tilde{z}^{(C)})^T \cdot (\mathcal{M}^{(A\to C)})^T \cdot \mathcal{L}^{(C)} \cdot \mathcal{M}^{(A\to C)} \cdot \mathcal{M}^{(C\to A)} \cdot \tilde{z}^{(C)} \tag{SI 114b}$$

$$= F^2 \cdot (\tilde{z}^{(C)})^T \cdot (\mathfrak{M}^{(A\to C)} \cdot \mathfrak{M}^{(C\to A)})^T \cdot \mathcal{L}^{(C)} \cdot \tilde{z}^{(C)} \tag{SI 114c}$$

$$= \kappa^{(C)} \tag{SI 114d}$$

Thus, the electric conductivity is invariant under changes of the designated species, and transforms as a "scalar" under the action of the transformation $\mathfrak{M}^{(A\to C)}$.

In contrast, the transformation of the transference numbers can only be derived implicitely from the transformation rule of the vector $\mathfrak{T}^{(A)}$. In particular, the invariance of the electric conductivity, and the transformation rules for the Onsager matrix and the valences imply that

$$\mathfrak{T}^{(A)} = F/\kappa^{(A)} \cdot \mathcal{L}^{(A)} \cdot \tilde{z}^{(A)} \tag{SI 115}$$

$$= F/\kappa^{(C)} \cdot (\mathfrak{M}^{(A\to C)})^T \cdot \mathcal{L}^{(C)} \cdot \mathfrak{M}^{(A\to C)} \cdot \mathfrak{M}^{(C\to A)} \cdot \tilde{z}^{(C)} \tag{SI 116}$$

$$= (\mathfrak{M}^{(A\to C)})^T \cdot \mathfrak{T}^{(C)}. \tag{SI 117}$$

Thus, $\mathfrak{T}^{(A)}$ transforms similar to the fluxes $\psi^{(A)}$. This conjugated transformation via transposed representation-matrices simplifies into two cases,

$$t_B^{(A)}|_{B\neq A,C} = \frac{\tilde{z}_B^{(A)}}{\tilde{z}_B^{(C)}} \cdot t_B^{(C)}, \tag{SI 118}$$

$$t_C^{(A)}|_{C\neq A} = -\sum_{D\neq C} \frac{M_D}{M_C} \cdot \frac{\tilde{z}_C^{(A)}}{\tilde{z}_D^{(C)}} \cdot t_D^{(C)}. \tag{SI 119}$$

However, since only N-2 transference numbers are independent, eq. (SI 118) suffices for the calculation of all parameters $t_B^{(A)}|_{B\neq A}$, from the parameters $t_B^{(C)}$. (This follows from the normalization $\tilde{z}^{(A)})^T \cdot \mathfrak{T}^{(A)} = 1/F$.) In particular, eq. (SI 118) can be supplemented by $t_C^{(A)} = 1 - \sum_{D\neq A,C} t_D^{(A)}$, such that eq. (SI 119) becomes redundant. Note that if the designated species $A$ refers to a neutral species ($z_A = 0$), then $\tilde{z}_B^{(A)} = z_B$, for all species $B \neq A$.

Finally, the diffusion matrix $\mathcal{D}^{(A)} = \mathcal{L}^{(A)} - \kappa \cdot \mathfrak{T}^{(A)} \otimes \mathfrak{T}^{(A)}$ transforms similar to the Onsager matrix,

$$\mathcal{D}^{(C)} = \left(\mathfrak{M}^{(C\to A)}\right)^T \cdot \mathcal{D}^{(A)} \cdot \mathfrak{M}^{(C\to A)}. \tag{SI 120}$$

### 4. *Example: Quaternary Electrolyte*

As example, we consider the quaternary electrolyte described in the main part. We define the fixed bijective assignment between the physical indices and the species-indices by

$$(A, B, C, D) = (H_2O, Ch^+, OAc^-, [Zn(OAc)_3]^-). \tag{SI 121}$$

In the main text we discussed numerical results obtained from simulations relative to the three different reference-species $H_2O$ (corresponds to $\alpha = 1$), $Ch^+$ (corresponds to $\alpha = 2$) and $[Zn(OAc)_3]^-$ (corresponds to $\alpha = 4$).

The numerical results for the transference numbers collected in table II can be validated by our analytical findings of this section. For this purpose we set the designated species appearing on the left side of eq. (SI 118) to $C = H_2O$, and calculate the corresponding parameters $t^{(A)}_{B\neq A}$ for the cases $A = Ch^+$, and $A = [Zn(OAc)_3]^-$ respectively. Since the designated species $C = H_2O$ is neutral, $\tilde{z}_B^{(H_2O)} = z_B$ for the three species $B \neq H_2O$. Using the data for $\tilde{z}_B^{(Ch^+)}$, $\tilde{z}_B^{([Zn(OAc)_3]^-)}$ and $t^{(H_2O)}_{B\neq A}$ comprised in table II, we find for the transference numbers relative to the designated species $A = Ch^+$

$$t^{(Ch^+)}_{OAc^-} = 0.129 \cdot (-1.570) \cdot (-1) = 0.203, \tag{SI 122a}$$

$$t^{(Ch^+)}_{[Zn(OAc)_3]^-} = 0.705 \cdot 3.330 = 2.350, \tag{SI 122b}$$

$$t^{(Ch^+)}_{H_2O} = 1 - t^{(Ch^+)}_{(OAc^-)} - t^{(Ch^+)}_{[Zn(OAc)_3]^-} = -1.560, \tag{SI 122c}$$

and for the transference numbers relative to the designated species $[Zn(OAc)_3]^-$,

$$t^{([Zn(OAc)_3]^-)}_{Ch^+} = 0.166 \cdot 1.430 = 0.237, \tag{SI 122d}$$

$$t^{([Zn(OAc)_3]^-)}_{OAc^-} = -1 \cdot 0.129 \cdot (-0.757) = 0.098, \tag{SI 122e}$$

$$t^{([Zn(OAc)_3]^-)}_{H_2O} = 1 - t^{([Zn(OAc)_3]^-)}_{(OAc^-)} - t^{([Zn(OAc)_3]^-)}_{Ch^+} = 0.665 \tag{SI 122f}$$

The values obtained in eqs. (SI 122a) to (SI 122f) for the transference numbers coincide almost exactly with the numerical results comprised in table II. The small discrepancies arise from the fact that the numerical results comprised in table II stem from averaging over the graphs in fig. 9. This validates our numerical results and proves consistency of the framework.

To illustrate the form of the representatation-matrices of the transformations described above, we state three transformations explicitely,

$$\mathfrak{M}^{(1\to 2)} = \begin{pmatrix} -M_1/M_2 & 0 & 0 \\ -M_3/M_2 & 1 & 0 \\ -M_4/M_2 & 0 & 1 \end{pmatrix}, \quad \text{and} \quad \mathfrak{M}^{(2\to 1)} = \begin{pmatrix} -M_2/M_1 & 0 & 0 \\ -M_3/M_1 & 1 & 0 \\ -M_4/M_1 & 0 & 1 \end{pmatrix} \tag{SI 123}$$

$$\mathfrak{M}^{(1\to 3)} = \begin{pmatrix} 1 & -M_2/M_3 & 0 \\ 0 & -M_1/M_3 & 0 \\ 0 & -M_4/M_3 & 1 \end{pmatrix}, \quad \text{and} \quad \mathfrak{M}^{(3\to 1)} = \begin{pmatrix} -M_2/M_3 & 0 & 0 \\ -M_1/M_3 & 1 & 0 \\ -M_4/M_3 & 0 & 1 \end{pmatrix}, \tag{SI 124}$$

$$\mathcal{M}^{(1\to4)} = \begin{pmatrix} 0 & 0 & -M_1/M_4 \\ 1 & 0 & -M_2/M_4 \\ 0 & 1 & -M_3/M_4 \end{pmatrix}, \quad \text{and} \quad \mathcal{M}^{(4\to1)} = \begin{pmatrix} -M_2/M_1 & 1 & 0 \\ -M_3/M_1 & 0 & 1 \\ -M_4/M_1 & 0 & 0 \end{pmatrix}. \tag{SI 125}$$

Thus, comparison of eqs. (SI 93) and (SI 123) shows that the transformation matrix $\mathcal{M}^{(2\to1)}$ is obtained from the mass-matrix in eq. (SI 93) by deleting the second column. This justifies using the same symbol for the two quantities.

### L. Formalizing Chemical Reactions

In general, chemical reactions occur both in the bulk electrolyte, and at the interfaces of electrolyte and active particles. Since we assume complete dissociation of the salts, we neglect bulk reactions and focus on surface reactions. These reactions serve as source-terms, and determine the interface conditions, which couple the solid phase with the electrolyte. We model surface reactions of an electrolyte species $\alpha$ by the expansion

$$r_\alpha = \sum_{k,\Gamma} a^\Gamma \nu_\alpha^k i_k^\Gamma. \tag{SI 126}$$

Here, $\nu_\alpha^k$ are the stoichiometric coefficients of reaction $k$. Here we set $\text{sign}(\nu_\alpha^k) = -1$ for reduction-reactions, and $\text{sign}(\nu_\alpha^k) = +1$, for reactions which increase the amount of species $\alpha$. Table SI 4 comprises the stoichiometric coefficients for the chemical reactions occurring in our simulations.

The surface reaction rates $i_k^\Gamma$ ([mol m$^{-2}$ s$^{-1}$]) measure the number of moles undergoing reaction $k$ per unit time, and unit surface area $a^\Gamma = A/V$ of the particular interface $\Gamma$. We model them using Butler-Volmer interface conditions,[18]

$$i^\Gamma = i_0^\Gamma \cdot \sinh\left(\frac{F z_{\mathrm{el}}^\Gamma}{2RT} \cdot \eta^\Gamma\right). \tag{SI 127}$$

Here, $z_{\mathrm{el}}^\Gamma$ denotes the electron-stoichiometry of the particular reaction. The offset $i_0^\Gamma$ and the overpotential $\eta^\Gamma$ are functions of salt-concentration. In particular, for a given surface reaction $\nu_\mathrm{A}\mathrm{A} + \nu_\mathrm{B}\mathrm{B} \rightleftharpoons \nu_\mathrm{C}\mathrm{C} + \nu_\mathrm{D}\mathrm{D}$, we define an oxidation-constant $a_{\mathrm{ox}} = (c_A/c_{A;0})^{|\nu_A|} \cdot (c_B/c_{B;0})^{|\nu_B|}$, and a reduction-constant $b_{\mathrm{red}} = (c_C/c_{C;0})^{|\nu_C|} \cdot (c_D/c_{D;0})^{|\nu_D|}$, where fractions $c_{A,B,C,D}/c_{A,B,C,D;0}$ serve as measure for the state of charge (SOC) of the species. For conversion electrodes, $c_A/c_{A;0} = 1$ ($c_A/c_{A;0} = 0$) implies that the electrode is completely charged (discharged) with species $A$. The offset is defined by $i_0^\Gamma = 2k^\Gamma \sqrt{a_{\mathrm{ox}} b_{\mathrm{red}}}$, where $k^\Gamma$ are constant reaction rates. We model the

overpotential by

$$\eta^{\Gamma} = \Phi_s^{\Gamma} - \Phi_l^{\Gamma} - U_0^{\Gamma} - \frac{RT}{F z_{\mathrm{el}}^{\Gamma}} \ln\left(\frac{a_{\mathrm{ox}}}{b_{\mathrm{red}}}\right). \tag{SI 128}$$

The potential difference $\Phi_s^{\Gamma} - \Phi_l^{\Gamma} - U_0^{\Gamma}$ is determined by the respective electrode-potential $\Phi_s^{\Gamma}$, the electric electrolyte potential $\Phi_l$, and the half-cell open circuit potential of the respective electrode $U_0^{\Gamma}$. We determine the equilibrium voltage $U_0^{\Gamma}(\mathrm{SOC})$ from the experimentally defined open-circuit discharge curve.

## SI 2. MODELLING OF ZINC ION BATTERY

### A. Electrolyte Composition

#### 1. *Reactions*

The electrolyte consists of choline actetate [Ch]OAc mixed with water, as to achieve liquid state. Zinc-acetate $Zn(OAc)_2$ is added as minor additive. We assume complete salt dissociation in the bulk,

$$[\mathrm{Ch}]\mathrm{OAc} \rightleftharpoons \mathrm{Ch}^{+} + \mathrm{OAc}^{-}, \tag{I-BULK}$$

$$3\mathrm{Zn(OAc)}_2 \rightleftharpoons \mathrm{Zn}^{2+} + 2[\mathrm{Zn(OAc)}_3]^{-}, \tag{II-BULK}$$

$$\mathrm{Zn(OAc)}_2 \rightleftharpoons \mathrm{Zn}^{2+} + 2\mathrm{OAc}^{-}. \tag{III-BULK}$$

Ionic choline does not participate in any other reaction. Further, secondary homogeneous reactions involve the formation of zinc-complexes from neutral zinc-acetate and from ionic species,

$$\mathrm{Zn}^{2+} + 3\mathrm{OAc}^{-} \rightleftharpoons [\mathrm{Zn(OAc)}_3]^{-}. \tag{IV-BULK}$$

Since zinc occurs mainly as $[Zn(OAc)_3]^-$ in the electrolyte,[19] we assume that $[Zn(OAc)_3]^-$ is the only zinc-species.

During discharging the cell, zinc dissolves from the zinc-anode, whereas, during charging of the cell, zinc gets deposited at the zinc-anode,[20] $\mathrm{Zn} \rightleftharpoons \mathrm{Zn}^{2+} + 2\mathrm{e}^{-}$. Dissolved $Zn^{2+}$-ions and negative bulk-ions $OAc^-$ form zinc-complexes via reaction-eq. (IV-BULK), where we neglect the inverse reaction-eq. (III-BULK). At the PBA-cathode, zinc-ions get inserted (extracted) into (from) the PBA-cathode during discharge (charge), $\mathrm{Zn}^{2+} + 2\mathrm{e}^{-} + [\mathrm{Fe(III)(CN)}_6] \rightleftharpoons [\mathrm{ZnFe(III)(CN)}_6]$.

Assuming that the formation of secondary zinc-acetate complexes is very fast and that the dominant secondary reaction is $[Zn(OAc)_3]^-$, we model the overall heterogeneous discharge reaction at the electrode-electrolyte interphases by

$$Zn + 3OAc^- \rightleftharpoons 2e^- + [Zn(OAc)_3]^-, \qquad \text{(I-INTERPHASE)}$$

$$[Zn(OAc)_3]^- + 2e^- + [Fe(III)(CN)_6] \rightleftharpoons 3OAc^- + [ZnFe(III)(CN)_6]. \qquad \text{(II-INTERPHASE)}$$

| Interphase solid/electrolyte | Species $\alpha$ | $\nu_\alpha^k$ | Type | Reaction |
|---|---|---|---|---|
| $\Gamma^{\text{anode}}$: Zinc-anode | $OAc^-$ | −3 | educt | Eq.(I-INTERPHASE) |
| | Zn | −1 | educt | Eq.(I-INTERPHASE) |
| | $[Zn(OAc)_3]^-$ | 1 | product | Eq.(I-INTERPHASE) |
| | $e^-$ | 2 | product | Eq.(I-INTERPHASE) |
| $\Gamma^{\text{cathode}}$: PBA-cathode | $OAc^-$ | 3 | product | Eq.(II-INTERPHASE) |
| | $[ZnFe(III)(CN)_6]$ | 1 | product | Eq.(II-INTERPHASE) |
| | $[Zn(OAc)_3]^-$ | −1 | educt | Eq.(II-INTERPHASE) |
| | $e^-$ | −2 | educt | Eq.(II-INTERPHASE) |

TABLE SI 4. Heterogeneous chemical reactions as product terms weighted by $\nu_\alpha^k$. The sign of stoichiometric coefficients $\nu_\alpha^k$ determines the type of reaction. Positive: product; negative: educt.

## 2. *Initial Concentrations*

For improving readability, we use the comprehensive notation $[\![X]\!] = c_X$ (with dimension $\text{mol}\,\text{m}^{-3}$),[21] and denote the total amount of species by the capital index "T". The reference electrolyte was prepared by dissolving 1.0 mol/L $Zn(OAc)_2$ in [Ch]OAc + 30 wt % water, implying a mass ratio of $b = m_{\text{water}}/m_{\text{[Ch]OAcWater}} = 0.3$.[22] The parameter for electrolyte mass density was provided by IoLiTec, $\rho_{\text{el}} = 1.35{\cdot}10^3\,\text{kg/m}^3$.[23] From this follow the initial concentrations of [Ch]OAc and water,

$$[\![\text{[Ch]OAc}]\!] = \frac{(1-b)\cdot\left(\rho - [\![Zn(OAc)_2]\!]\cdot M_{Zn(OAc)_2}\right)}{M_{\text{[Ch]OAc}}},$$

$$[\![\text{water}]\!] = \frac{b\cdot\left(\rho - [\![Zn(OAc)_2]\!]\cdot M_{Zn(OAc)_2}\right)}{M_{\text{water}}}. \qquad \text{(SI 129)}$$

Assuming complete dissociation, then determines the initial concentrations of the charged species, $[\![Ch^+]\!] = [\![[Ch]OAc]\!]_T$ and $[\![[Zn(OAc)_3]^-]\!] = [\![Zn(OAc)_2]\!]_T$. Using electroneutrality, $[\![OAc^-]\!] = [\![Ch^+]\!] - [\![[Zn(OAc)_3]^-]\!] = [\![[Ch]OAc]\!]_T - [\![Zn(OAc)_2]\!]_T$. For a collection of the values see Table SI 6.

### 3. *Partial Molar Volumes*

We model the set of partial molar volumes by constant values, $\nu_{water}, \nu_{Ch^+}, \nu_{OAc^-}, \nu_{[Zn(OAc)_3]^-}$. Due to the electrolyte equation of state, eq. (60), only three molar volumes are independent since all initial concentrations are known. Structure-formulas for the complexes can be found in Table SI 5. The partial molar volume of water is calculated by $\nu_{water} = M_{water}/\rho_{water}$. We assume that

| Species | Structure Formula |
|---|---|
| Choline acetate | $[Ch]OAc$: $C_7H_{17}NO_3$ |
| Zinc acetate | $Zn(OAc)_2$: $ZnC_4H_6O_4$ |
| Choline | $Ch^+$: $C_5H_{14}NO$ |
| Acetate | $OAc^-$: $C_2H_3O_2$ |
| Charged zinc-acetate complex | $[Zn(OAc)_3]^-$: $ZnC_6H_9O_6$ |

TABLE SI 5. Molecular complexes in the electrolyte.

the $Ch^+$-ion is "larger" than the $OAc^-$-ion, $\nu_{OAc^-} = n_R \cdot \nu_{Ch^+}$, where we set $n_R \approx 0.8$. We use the electrolyte described in Ref. 24 and set the partial molar volume of $[Zn(OAc)_3]^-$ to the partial molar volume of zincate from this reference. This fixes

$$\nu_{Ch^+} = \frac{1 - c_{water}\nu_{water} - c_{[Zn(OAc)_3]^-}\nu_{[Zn(OAc)_3]^-}}{c_{Ch^+} + 0.8 \cdot c_{OAc^-}}. \tag{SI 130}$$

Table SI 7 comprises the values for all partial molar volumes.

### 4. *Viscosity*

The viscosity of the as-prepared initial electrolyte composition was provided by IoLiTec ($\eta$ = 25.3 mPa s).[23]

| Parameter | Species | Value | Source |
|---|---|---|---|
| $b$ | Relative water content (wt % water in neat IL) | $3.00{\cdot}10^{-1}$ | 22 |
| Mass density ρ / kg m$^{-3}$ | Electrolyte solution | $1.35{\cdot}10^{3}$ | 23 |
| Concentrations $c_\alpha$ / mol m$^{-3}$ | $[\![Zn(OAc)_2]\!]_T$ | $1.00{\cdot}10^{3}$ | 22 |
| | $[\![[Ch]OAc]\!]_T$ | $5.00{\cdot}10^{3}$ | calc. |
| | $[\![H_2O]\!]_T$ | $19.43{\cdot}10^{3}$ | calc. |
| | $[\![Ch^+]\!]$ | $5.00{\cdot}10^{3}$ | calc. |
| | $[\![OAc^-]\!]$ | $4.00{\cdot}10^{3}$ | calc. |
| | $[\![[Zn(OAc)_3]^-]\!]$ | $1.00{\cdot}10^{3}$ | calc. |
| Electrolyte viscosity $\eta$ / kg m$^{-1}$ s$^{-1}$ | Electrolyte | $2.53{\cdot}10^{-2}$ | 23 |
| | Reference (water) | $0.89{\cdot}10^{-3}$ | 25 |

TABLE SI 6. Initial composition of the electrolyte and electrolyte parameters.

### 5. *Transport Parameters: Modelling Onsager Matrix*

Six independent transport parameters exist in a quaternary electrolyte; the electric conductivity $\kappa$, the two transference numbers $t_3, t_4$, and the three diffusion coefficients $\mathcal{D}_{33}, \mathcal{D}_{34}, \mathcal{D}_{44}$. These parameters are all functions of the Onsager-matrix $\mathcal{L}$. We assume that this matrix has diagonal form, and model the components by $\mathcal{L}_\alpha = Đ_\alpha c_\alpha / RT$, where $Đ_\alpha(c_\beta)$ are the hydrodynamical diffusion coefficients. These are defined by the Stokes-Einstein relation $Đ_\alpha = k_B T / 6\pi r_\alpha \eta$, where $r_\alpha$ are the ionic radii, and $\eta$ is the viscosity. We eliminate the inaccessible volume-term using dilute coefficients $Đ_\alpha^{\text{dilute}} = RT\lambda_\alpha^{\text{dilute}} / F^2 z_\alpha$, where $\lambda_\alpha^{\text{dilute}}$ are the limiting equivalent conductivities under indefinite dilution. Thus, we find $\mathcal{L}_{\text{ion}} = \eta^{\text{dilute}} \lambda_{\text{ion}}^{\text{dilute}} c_{\text{ion}} / F^2 \eta |z_{\text{ion}}|$. The electrolyte viscosity $\eta$ was measured by IoLiTec,[23] and water was taken as reference for the dilute viscosity $\eta^{\text{dilute}}$. For specific data, see table table SI 6.

| Parameter | Species | Value | Source |
|---|---|---|---|
| Mass density $\rho$ / kg m$^{-3}$ | Water | $9.97{\cdot}10^{2}$ | 26 |
| Partial molar volumes $\nu_\alpha$ / m$^3$ mol$^{-1}$ | Water | $1.80{\cdot}10^{-5}$ | calc. |
| | Choline ion | $6.93{\cdot}10^{-5}$ | calc. |
| | Acetate ion | $5.55{\cdot}10^{-5}$ | calc. |
| | Zinc acetate ion | $8.00{\cdot}10^{-5}$ | 24 |
| Equivalent conductivity $\lambda_\alpha^{\text{dilute}}$ / S m$^2$ mol$^{-1}$ | Choline ion | $42.00{\cdot}10^{-4}$ | 27 |
| | Acetate ion | $40.89{\cdot}10^{-4}$ | 25 |
| | Zinc ion | $105.60{\cdot}10^{-4}$ | 25 |
| Viscosity $\eta$ / kg m$^{-1}$ s$^{-1}$ | Electrolyte | $25.30{\cdot}10^{-3}$ | 23 |
| | Reference (water) | $0.89{\cdot}10^{-3}$ | 25 |

TABLE SI 7. Parameters of the electrolyte-species.

## B. Electrodes

### 1. *Solid Phase Equations*

We model a zinc foil by setting appropriate boundary conditions for the flux density of zincate ions with a Butler-Volmer reaction (see eq. (SI 127)). The PBA cathode is porous and we apply porous electrode theory.[28] Thus, the primary variables of the solid-phases are the zinc concentration, and the half-cell-voltage of the cathode ($c_{\text{Zn}}^{\text{PBA}}$, $\Phi^{\text{PBA}}$). We neglect zinc diffusion in the cathode. Thus, the loss of salt in the liquid-phase, determined by the reaction rate $r_{\text{Zn}}$ via eq. (SI 126), equals the cathode-concentration of zinc, $\partial_t c_{\text{Zn}}^{\text{PBA}} = -r_{\text{Zn}}^{\text{PBA}}/(1-\varepsilon^{\text{PBA}})$. However, here we use the weighted expression $c_{\text{Zn}}^{\text{PBA}}/c_{\text{Zn}}^{\text{PBA;max}}$ as primary variable, where $c_{\text{Zn}}^{\text{PBA;max}} = 1$ corresponds to a fully charged cathode. This ratio determines the state-of-charge (SOC) of the cathode,

$$\partial_t \text{SOC}^{\text{PBA}} = -\frac{r_{\text{Zn}}^{\text{PBA}}}{(1-\varepsilon^{\text{PBA}})c_{\text{Zn}}^{\text{PBA;max}}}. \qquad \text{(SI 131)}$$

Furthermore, we set the cell-voltage of the porous zinc-anode to zero, and determine the cell-voltage of the PBA-cathode implicitely from the cathode-reaction rate $r_\alpha^{\text{PBA}}(\Phi^{\text{PBA}})$ using the Faradaic interface condition SI 133,

$$0 = \Phi^{\text{anode}}, \qquad \text{(SI 132)}$$

$$0 = I + \int \mathrm{d}x \sum_{\alpha=1}^{N} F z_\alpha r_\alpha^{\mathrm{PBA}}(\Phi^{\mathrm{PBA}}). \tag{SI 133}$$

### 2. *Electrode Parameters*

We assume constant volume fractions of the zinc-anode, separator and PBA-cathode, and estimate the volume fractions of anode and separator ($\varepsilon_{a,s} = 0.3$). From the experimental data,[29] we calculated the volume fraction of the PBA-cathode, $\varepsilon_{\mathrm{solid}} = V_{\mathrm{PBA}}/V_{\mathrm{cathode}}$. The volume of the cathode is $V_{\mathrm{cathode}} = l \cdot A_{\mathrm{cathode}}$, where $l$ is the length of cathode and $A_{\mathrm{cathode}}$ is the cathode-surface-area. Furthermore, we calculated the volume of the PBA using the mass loading $m_{\mathrm{load}}$, the surface area $A_{\mathrm{cathode}}$ and the mass denisity of the PBA-material $\rho_{\mathrm{PBA}}$, via $V_{\mathrm{PBA}} = m_{\mathrm{load}} \cdot A_{\mathrm{cathode}}/\rho_{\mathrm{PBA}}$. Altogether, $\varepsilon_{\mathrm{solid}} = m_{\mathrm{load}}/\rho_{\mathrm{PBA}} l \approx 0.7407$. Thus , the volume fraction of the liquid phase in the PBA-cathode is $\varepsilon = 1 - \varepsilon_{\mathrm{solid}} = 0.2593$. The ratio of host-sites of the PBA-cathode, to sites available in the PBA-cathode which can be filled by zinc, is four-to-one.[30] Thus, the maximal zinc-concentration in the PBA-cathode is $c_{\mathrm{Zn}}^{\max} = \rho_{\mathrm{PBA}}/(4M_{\mathrm{PBA}})$. We summarize the electrode-parameters in table SI 8.

| Parameter | Electrode | Value | Source |
|---|---|---|---|
| Specific surface area $a$ / $\mathrm{m}^{-1}$ | Anode | $1.0{\cdot}10^{5}$ | Fit parameter |
| | Cathode | $1.0{\cdot}10^{4}$ | Fit parameter |
| Reaction rate $k$ / $\mathrm{mol\,m^{-2}\,s^{-1}}$ | Anode | $1.0{\cdot}10^{-7}$ | Fit parameter |
| | Cathode | $1.0{\cdot}10^{-7}$ | Fit parameter |
| Volume fraction $\varepsilon$ | Anode | $3.0{\cdot}10^{-1}$ | Fit parameter |
| | Separator | $3.0{\cdot}10^{-1}$ | Fit parameter |
| | Cathode | $2.6{\cdot}10^{-1}$ | Calculated |
| Mass loading $m_{\mathrm{load}}$ / $\mathrm{kg\,m^{-2}}$ | Cathode | $9.5{\cdot}10^{-2}$ | 29 |
| Thickness $l$ / $\mathrm{m}^{-1}$ | Cathode | $1.5{\cdot}10^{-4}$ | 29 |
| Mass density $\rho_{\mathrm{PBA}}$ / $\mathrm{kg\,m^{-3}}$ | Cathode | $1.8{\cdot}10^{3}$ | 29 |

TABLE SI 8. Battery-Parameters.

### C. Implementation: Computational Details

We implement the system of transport equations in a one-dimensional finite-volume model in MATLAB. The grid points are erected with finite step-size ($\Delta x = 2.8\,\mu\text{m}$) and the corresponding domain of length $L_{\text{cell}} = 300\,\mu\text{m}$ consists of the zinc anode ($x = [0; 150\,\mu\text{m}]$), followed by the separator ($x = [150\,\mu\text{m}; 200\,\mu\text{m}]$) and the PBA-cathode ($x = [200; L_{\text{cell}}]$). As numerical solver we use the fully implicit ode15i MATLAB-solver for differential algebraic equations. Relative and absolute tolerances were both set to $10^{-6}$.

## SI 3. SIMULATION RESULTS

In this section we present supporting material for the discussion of the simulation results, given in the main text.

### A. Electrolyte Dynamics

Figure SI 1 comprises simulation results for the electrolyte-dynamics by application of a moderate discharge current ($I = 0.1\,\text{mA}\,\text{cm}^{-2}$). Subfig. SI 1a) illustrates the complete discharge profile over time and highlights the designated discharge moments. The evolution of the electrolyte electric potential $\Phi$ is shown in sub-fig. SI 1b). Apparently, $\Phi$ exhibits a gradient from anode to cathode, which remains constant at $\Delta\Phi \approx 1\,\text{mV}$ during discharge. Thus, the anode is more electropositive than the cathode, which implies that the $OAc^-$-/ and $[Zn(OAc)_3]^-$-anions ($Ch^+$-cations) experience a migrational pull towards the anode (cathode) during discharge. Sub-fig. SI 1c)-f) illustrate the evolution of the specific volume-fractions $\nu_\alpha c_\alpha$. These comprise the dynamics of the species concentrations $c_\alpha$, since the partial molar volumes are assumed constant. In addition, we collect the directions of the species-velocities $\mathbf{v}_\alpha$ during discharge in table SI 9.

A common behaviour in the evolution of $\mathbf{v}, c_\alpha, \Phi, \mathbf{v}_\alpha$ can be read off from these subfigures and the table. All quantities exhibit an inital dynamical phase in which characteristic profiles emerge, before attaining a quasi-stationary state. Notably, the transient times of the quantities coincide. These observations suggest the interpration given in the main text. Our simulations start with a homogeneous electrolyte profile where all quantities $\mathbf{v}, c_\alpha, \Phi, \mathbf{v}_\alpha$ are constant (table SI 7). This constitutes a static equilibrium state of the system. By application of external currents $j$, the system is pushed out of equilibrium. However, as the system equilibrates towards a locally stable

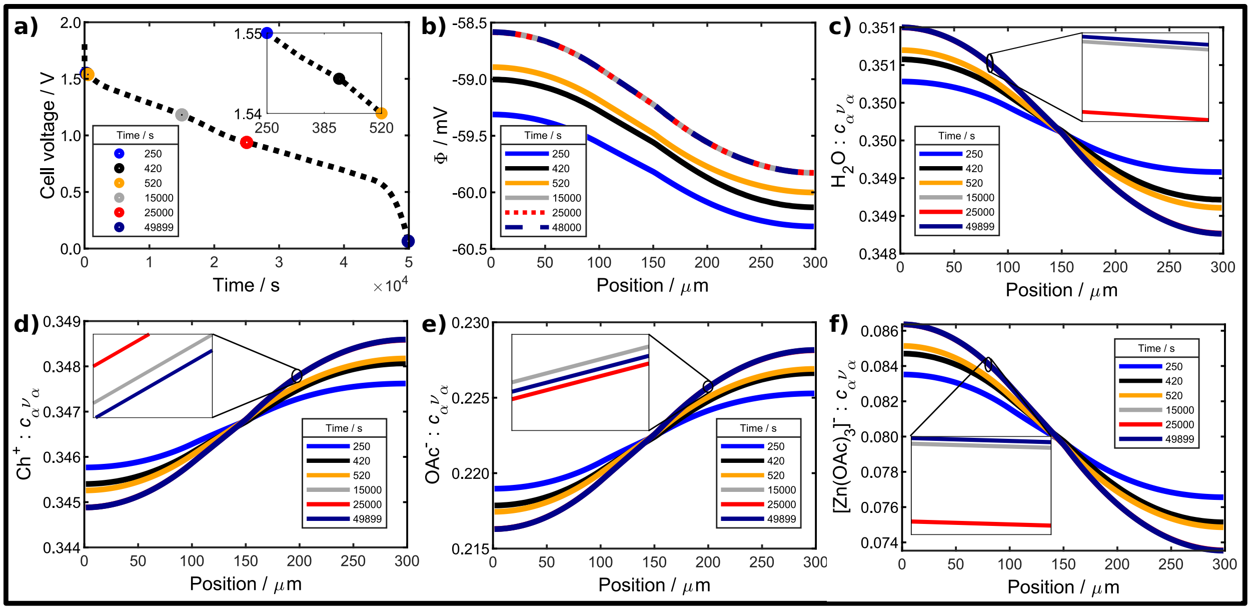


FIG. SI 1. **a)** Cell voltage of the complete discharge over discharge time. The colored dots specifiy designated moments of discharge. **b)** Electrolyte electric potential at designated moments exhibits that the anode is more positive than the cathode. **c)-f)** Volume fractions of the electrolyte species. Insets show quasi-stationary profiles once the electrolyte has relaxed towards quasi-equilibrium ($t \gtrsim 1000\,\mathrm{s}$)

.

state, the quantities $\mathbf{v}$, $c_\alpha$, $\Phi$, $\mathbf{v}_\alpha$ experience a “dynamical” phase. Convection and species velocities change direction, and gradients in the electrolyte electric potential and the species concentrations build up. After some transient time, the system attains a quasi-stationary state and the quantities almost remain constant.

We probe this interpretation by a detailed study of the evolution of each electrolyte-species, and it’s implication on the overall dynamics.

The concentration of the nagative zinc-complex increases at the anode and decreases at the cathode (fig. SI 1f)), although there is a net flux of $[Zn(OAc)_3]^-$ towards the cathode at all times (table SI 9). Simultaneously, according to the reaction eq. (I-INTERPHASE), dissolution of zinc from the anode produces $[Zn(OAc)_3]^-$ near the anode. Thus, the net increase of $[Zn(OAc)_3]^-$-concentration at the anode during the transient-phase suggests that production by reactions dominates over transport of $[Zn(OAc)_3]^-$ towards the cathode. This transport is crucial for the operation of the cell, as the zinc-complex is intercalated into the cathode-structure. After the transient-phase, loss due to transport and gain due to production balance, and the concentration profiles becomes quasi-

stationary. Furthermore, the net flux of $[Zn(OAc)_3]^-$-ions towards the cathode at all times reveals that diffusion towards the cathode, due to stark concentration gradients, dominates over migration, which pushes $[Zn(OAc)_3]^-$-anions toward the more electro-positive anode (table SI 9).

We make a similar observation for the dynamics of the $OAc^-$-ions. Initially, the local production of $OAc^-$-ions at the cathode in the course of zinc-intercalation, reaction eq. (II-INTERPHASE), dominates over the flux of $OAc^-$-ions towards the cathode (table SI 9). After the transient-phase, both competing processes are in quasi-equilibrium. The negative flux of $OAc^-$-ions is the result of diffusion and migration, which both push the $OAc^-$-ions towards the anode.

The $Ch^+$-ions are pushed towards the more electronegative cathode by migration. The velocity-profiles exhibits a highly non-homogeneous characteristics during the transient phase, and becomes stable when quasi-equilibrium is attained (table SI 9). During the transient phase, $Ch^+$-ions move towards the cathode, and then converge into a net flux towards the anode.

The highly non-homogeneous velocity-profile of water during the transient phase (table SI 9), suggests that water species serve as a local supply for volume-compensation. In our model, water has by far the lowest partial molar volume (see table SI 7), and is abundant compared to the ionic species ( table SI 6). Furthermore, water serves as designated species, $\tilde{z}_{H_2O} = 0$. As consequence, water effectively balances local volume-inhomogeneities.

These observations suggest that the overall profile for the center-of-mass convection is the result of species-transport, and volume-effects due to species-production. Although, in our model, $[Zn(OAc)_3]^-$-ions have the largest partial molar volume, $OAc^-$-ions are the dominant species with respect to volume-production (table SI 7); the consumption of one $[Zn(OAc)_3]^-$-ion per cathode reaction produces three $OAc^-$-ions at the cathode. Thus, this reaction consumes a net-molar-volume of $3\nu_{OAc^-} - \nu_{[Zn(OAc)_3]^-} > 0$. This amount of volume attained by the $OAc^-$-ions is at disposal for displacement by bulk-electrolyte. The same, “inverse” process occurs at the anode. Here, in each reaction a net amount of volume is produced, which is then filled by bulk electrolyte. Thus, both electrode-reactions promote an advective flux towards the cathode, as long as reactions dominate over transport. This is exactly the case during the transient phase, where the center-of-mass velocity is indeed negative. Once the reactions are in equilibrium with transport, convection is the delicate trade-off between transient currents. The insets shown in fig. SI 1 illustrate that the quasi-stationary state still exhibits small dynamics.

| Electrol. dynamics | Moment $t/s$ | Direction $\mathbf{v}_{H_2O}$ | Direction $\mathbf{v}_{Ch^+}$ | Direction $\mathbf{v}_{OAc^-}$ | Direction $\mathbf{v}_{[Zn(OAc)_3]^-}$ |
|---|---|---|---|---|---|
| Transient phase | 250 | chaotic/mixed | cathodic | anodic | cathodic |
| | 420 | chaotic/mixed | cathodic | anodic | mixed; mainly cathodic |
| | 520 | chaotic/mixed | cathodic | anodic | cathodic |
| Quasi-stationarity | 15000 | anodic | anodic | anodic | cathodic |
| | 25000 | anodic | anodic | anodic | cathodic |
| | 49899 | anodic | anodic | anodic | cathodic |

TABLE SI 9. Species veolicities $\mathbf{v}_\alpha$ at different moments of discharge. The anodic direction corresponds to a negative convection-profile, whereas the cathodic direction corresponds to a positive convection profile.

### 1. *High Discharge Current*

Figure SI 2a)-c) show the simulation results of cell-discharge via the enhanced discharge current $I = 10\,\mathrm{mA\,cm^{-2}}$. Subfigure a) shows the profile of the cell-voltage during the complete discharge, and highlights designated moments. Subfigures b) and c) illustrate the evolution of the zinc-complex and of the center-of-mass convection.

Apparently, the capacity of the cell is highly reduced, compared to the capacity obtained by using moderate discharge currents (see fig. 3). This suggests a premature breakdown of the cell-operation due to enhanced electrolyte dynamics. From subfigure b) shows complete salt-depletion near the cathode at end of discharge. Thus, the mandatory cathode-reaction cannot sustain cell-operation anymore due to reactand depletion, and the discharging stops. Subfigure c) exhibits enhanced dynamics for the large discharge current. Towards the end of discharge, convection diminishes at the cathode. Following the discussion of the previous section, we suggest that this is a consequence of reactant-depletion. Since no more $OAc^-$-ions are formed near the cathode, the volumetric stimulus for convection breaks down.

### 2. *Various Currents*

Figure 8 and subfigures d)-f) in fig. SI 2 show the profiles of the species concentrations at end of discharge for the discharge currents $I$=$0.1\,\mathrm{mA\,cm^{-2}}$, $2\,\mathrm{mA\,cm^{-2}}$, $3\,\mathrm{mA\,cm^{-2}}$, $4\,\mathrm{mA\,cm^{-2}}$

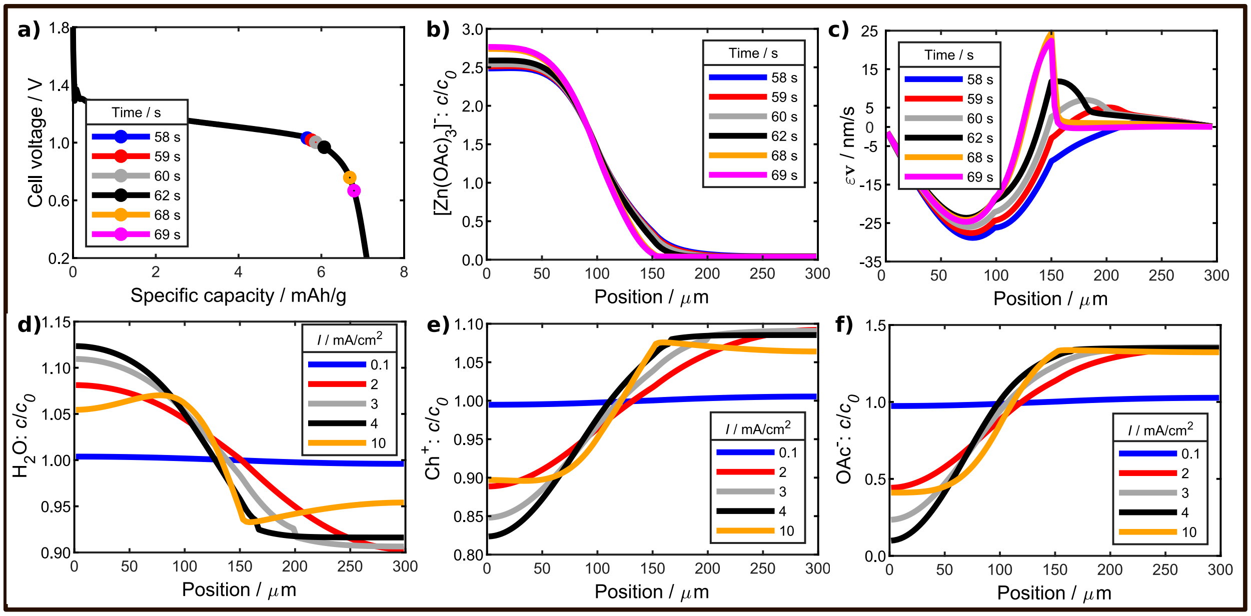


FIG. SI 2. Detailed investigation for discharge current density $I = 10\,\mathrm{mA\,cm^{-2}}$. Subfigure a) shows the complete discharge of the cell and designated moments of discharge (colored points). Subfigure b) shows the concentration profile of $[Zn(OAc)_3]^-$-ions at the designated moments. Subfigure c) shows the convection profile at the designated moments. Subfigures d)-f) show concentration profiles at end of discharging for different discharge currents.

and $10\,\mathrm{mA\,cm^{-2}}$. For all but the highest discharge current, the gradients in the profiles increase with increasing currents. Therefore, for these currents, increasing the discharge dynamics leads to enhanced profiles in the species concentrations.

Notably, the gradients are most significant at the discharge current $I = 4\,\mathrm{mA\,cm^{-2}}$, whereas, in principle, one would expect that the gradients become most profound for the highest discharge current. However, our observations from the previous section are in accordance with this effect, and a simple expalanation can be given. The enhanced dynamics at $I = 10\,\mathrm{mA\,cm^{-2}}$ leads to the breakdown of cell-operation due to salt depletion near the cathode. In particular, the breakdown is reached sufficiently fast (roughly after 7 s), such that the profile has not enough time to increase the $[Zn(OAc)_3]^-$-concentration at the anode any further. This is confirmed by fig. SI 2b) which shows that the $[Zn(OAc)_3]^-$-concentration near the anode increases monotonously until end of cell-operation, and does not attain a quasi-stationary state.

Therefore, increasing the discharge dynamics leads to enhanced profiles in the species concentrations and the electrolyte exhibits increasingly non-trivial convection profiles. However, once the

dynamics become too fast, cell operation breaks down because the interplay of diffusion, migration and convection becomes unstable for cell-operation.

### B. Consistency Check: Varying Reference Species

We probe consistency of our framework by performing equal discharge simulations ($I = 0.1\,\mathrm{mA\,cm^{-2}}$) within the different frames collected in table II. To extend this examination to differing length-scales, we compare simulation results of microscopic and mesoscopic quantities obtained from the three frames.

To make the implementations consistent with each other, we must take account for the fact that the representations of the Onsager matrices in the three different frames cannot be chosen independently. Thus, we apply the transformation rules discussed in section SI 1 K on the first frame, and obtain thereby the correct matrices $\mathcal{L}$ in the two other frames.

Subfigure SI 3a) shows cell-voltage over discharge time, for each reference-frame. Apparently, the results agree quantitatively with very high accuracy. Cell voltage is a mesoscopic quantity, which is easily accessible to experimental measurements. Thus, the mesoscopic behaviour of the system in the three different frames is consistent.

Subfigure SI 3b) illustrates the concentration profile of the $[Zn(OAc)_3]^-$-ions at end of discharge, for two different frames of reference. Agreement of the results in both frames proves consistency of miscroscopic simulation-results. In particular, note that the $[Zn(OAc)_3]^-$-ions are a designated species in the second frame.

Subfigure SI 3c) quantifies this agreement. Apparently, the relative error between the results illustrated in subfigure b) is of order $10^{-8}$, and thus lies within numerical accuracy of the simulations (see section SI 2 C). This confirms that the framework delivers consistent results, independent of the choice of designated species.

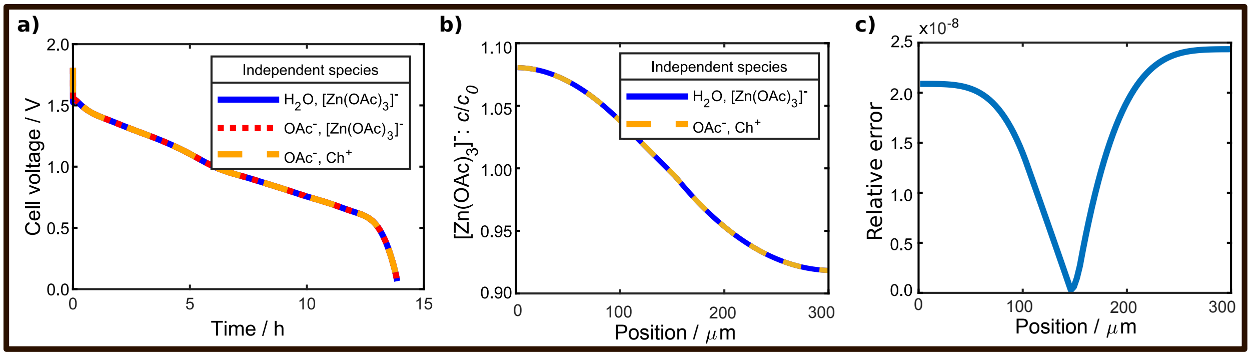


FIG. SI 3. Comparison of simulation results for different reference-species. Subfigure a) shows the discharge profile for three different reference-species. Subfigure b) shows the concentration profile of the $[Zn(OAc)_3]^-$-ions at end of discharge in two different reference frames. Subfigure c) shows the relative error of the concentrations of $[Zn(OAc)_3]^-$-ions at end of discharge for the two reference frames with independent species ($H_2O$, $[Zn(OAc)_3]^-$) and ($OAc^-$, $[Zn(OAc)_3]^-$).

---


[1] G. Lebon, D. Jou, and J. Casas-Vázquez, *Understanding non-equilibrium thermodynamics*, Vol. 295 (Springer, 2008).

[2] I. Müller, Archive for Rational Mechanics and Analysis **45**, 241 (1972).

[3] W. Dreyer, C. Guhlke, and R. Müller, Entropy **20**, 939 (2018).

[4] K. Henjes, Annals of Physics **223**, 277 (1993).

[5] I. Müller, *A history of thermodynamics: the doctrine of energy and entropy* (Springer Science & Business Media, 2007).

[6] S. Kovetz and A. Kovetz, *Electromagnetic Theory*, Oxford science publications (Oxford University Press, 2000).

[7] I. Liu, *Continuum Mechanics*, Advanced Texts in Physics (Springer Berlin Heidelberg, 2002).

[8] W. Noll, Archiv der Mathematik **21**, 87 (1970).

[9] C. De Boor, Journal of Elasticity **15**, 225 (1985).

[10] L. Martins, Journal of elasticity **54**, 89 (1999).

[11] D. Bothe and W. Dreyer, Acta Mechanica **226**, 1757 (2015).

[12] C. Guhlke, Ph.D. thesis, TU-Berlin, Berlin, Germany (2015).

[13] K. Binnemans, Chemical Reviews **105**, 4148 (2005).

[14] A. Latz and J. Zausch, Beilstein Journal of Nanotechnology **6**, 987 (2015).

[15] B. R. Sundheim, The Journal of Physical Chemistry **60**, 1381 (1956).

[16] W. Dreyer, C. Guhlke, and R. Müller, Phys. Chem. Chem. Phys. **17**, 27176 (2015).

[17] G. K. Batchelor, *An Introduction to Fluid Dynamics*, Cambridge Mathematical Library (Cambridge University Press, 2000).

[18] A. Latz and J. Zausch, Electrochimica Acta **110**, 358 (2013).

[19] P. D. Vreese, A. Skoczylas, E. Matthijs, J. Fransaer, and K. Binnemans, Electrochimica Acta **108**, 788 (2013).

[20] C. Xu, B. Li, H. Du, and F. Kang, Angewandte Chemie International Edition **51**, 933 (2012).

[21] S. Clark, A. Latz, and B. Horstmann, ChemSusChem **10**, 4735 (2017).

[22] Z. Liu, G. Pulletikurthi, and F. Endres, ACS Applied Materials & Interfaces **8**, 12158 (2016), pMID: 27119430.

[23] IoLiTec Ionic Liquids Technologies Gmbh, Private Communication (2017).

[24] J. Stamm, A. Varzi, A. Latz, and B. Horstmann, Journal of Power Sources **360**, 136 (2017).

[25] M. L. Williams, *CRC Handbook of Chemistry and Physics, 76th edition*, Vol. 53 (BMJ Publishing Group, 1996) pp. 504–504.

[26] J. A. Riddick, W. B. Bunger, and T. K. Sakano, *Organic solvents: physical properties and methods of purification* (John Wiley and Sons, New York, NY, 1986).

[27] R. Fleming, Journal of the Chemical Society (Resumed) , 4914 (1960).

[28] T. Schmitt, A. Latz, and B. Horstmann, Electrochimica Acta **333**, 135491 (2020).

[29] Z. Liu, P. Bertram, and F. Endres, Journal of Solid State Electrochemistry **21**, 2021 (2017).

[30] S. Liu, W. Han, B. Cui, X. Liu, F. Zhao, J. Stuart, and S. Licht, Journal of Power Sources **342**, 435 (2017).
